# Supplementary material for: Interpretational errors in statistical causal inference
Source: arXiv:2312.07610 source file (2023-12-11)
Supplement: Supplementary file 1 [file AppendixA_ProofDynGform.tex]

\section{Proofs}

For the following results, we consider a longitudinal data structure identical to that elaborated in Section \ref{sec: case2}. However, for increased generality and concordance with the Single World Intervention Graph (SWIG) theory developed by \citetSM{Richardson2013}, we will consider a more general causal model defined by the following propositions:

Let $\mathbf{V} \equiv \{O, H\}$ be a set of observed and hidden random variables and consider a directed acyclic graph $\mathcal{G}$ with nodeset $V$ and topological order $(H_0, L_0,A_0, \ldots, H_{J-1},L_{J-1}, A_{J-1}, Y)$. 

\begin{definition}[Counterfactual existence assumption]\label{def: CEA}
\ \begin{itemize}
    \item [$(i)$] For each variable $V \in \mathbf{V}$ and assignment $\mathbf{\tilde{pa}}$ to $pa_{\mathcal{G}}(V)$, the parents of
$V$ in $\mathcal{G}$, we assume the existence of a counterfactual variable $V (\mathbf{\tilde{pa}})$.
    \item [$(ii)$] For any set $\mathbf{R}$, with $\mathbf{R}\neq pa_{\mathcal{G}}(V)$, $V(\tilde{\mathbf{r}})$ is defined recursively via:
    \begin{align*}
        V(\tilde{\mathbf{r}}) = V\Bigg(\tilde{\mathbf{r}}_{(pa_{\mathcal{G}}(V) \cap \mathbf{R})}, (\mathbf{PA}_V\setminus \mathbf{R})(\mathbf{\tilde{r}})\Bigg)
    \end{align*}
        where $(\mathbf{PA}_V\setminus \mathbf{R})(\mathbf{\tilde{r}}) \equiv \{V^*(\tilde{\mathbf{r}}) \mid V^*\in pa_{\mathcal{G}}(V), V^*\not\in \mathbf{R}\}$, and where we let $\mathbb{V}(\mathbf{\tilde{r}}) \equiv \{{V}(\mathbf{\tilde{r}}) \mid V\in\mathbf{V}\}.$
\end{itemize}

\end{definition}

\begin{definition}[FFRCISTG Independence Assumption]\label{def: FFRind}
For every $\mathbf{v}^{\dagger}$, the variables

\begin{align*}
    \{V(\mathbf{pa}_V^{\dagger}) \mid V\in\mathbf{V}, \mathbf{pa}_V^{\dagger} = \mathbf{v}^{\dagger}_{pa_{\mathcal{G}}(V)}\}
\end{align*}
 are mutually independent.
\end{definition}

We define SWIGs $\mathcal{G}(\mathbf{a}^{\dagger})$ and d-SWIGs $\mathcal{G}(g)$  as constructed in \citetSM{Richardson2013}.

\begin{definition}[Factorization]
A joint distribution $P(\mathbb{V}(\mathbf{\tilde{a}})$ factorizes with respect to a SWIG $\mathcal{G}(\mathbf{a}^{\dagger})$ if 
\begin{align*}
    P(\mathbb{V}(\mathbf{\tilde{a}}) = \prod\limits_{Y\in\mathbf{V}}P(Y(\mathbf{\tilde{a}}_Y \mid \mathbb{pa}_{\mathcal{G}, Y}(\mathbf{\tilde{a}}) \setminus \mathbb{A}(\mathbf{\tilde{a}})),
\end{align*}
whenever the right hand side is well-defined and where $$\mathbb{pa}_{\mathcal{G}, Y}(\mathbf{\tilde{a}}) \setminus \mathbb{A}(\mathbf{\tilde{a}}) = \{V(\mathbf{\tilde{a}}_V) \mid V\in pa_{\mathcal{G}}(Y)\setminus\mathbf{A}\}.$$ \end{definition}

\begin{definition}[Modularity]
Pairs $(\mathcal{G}, P(\mathbf{V}))$ and $(\mathcal{G}(\tilde{\mathbf{a}}), P(\mathbb{V}(\tilde{\mathbf{a}})))$ are said to satisfy the modularity property if for every $Y\in\mathbf{V}$, 
\begin{align*}
  &  P(Y(\tilde{\mathbf{a}}_Y)=y \mid (pa_{\mathcal{G}(\tilde{\mathbf{a}})}(Y(\tilde{\mathbf{a}})\setminus\tilde{\mathbf{a}}) = \mathbf{q}) \\
  = & P(Y=y \mid (pa_{\mathcal{G}}(Y)\setminus \mathbf{A}) = \mathbf{q}, (pa_{\mathcal{G}}(Y)\cap \mathbf{A}) = \tilde{\mathbf{a}}_{a_{\mathcal{G}}(Y)\cap \mathbf{A}}),
\end{align*} 
whenever both sides are well-defined.
\end{definition}

\begin{lemma}[Lemma 49 from \citetSM{Richardson2013}] \label{lemma49}

If $P(\mathbf{V})$ and $P(\mathbb{V}(\mathbf{a}^{\dagger}))$ factorize and obey modularity with respect to $\mathcal{G}$ and $\mathcal{G}(\mathbf{a}^{\dagger})$, then for any $\mathbf{W}\subseteq \mathbf{V}\setminus \mathbf{A} $ $$P(\mathbb{W}(\mathbf{a}^{\dagger}) = \mathbf{w}, \mathbb{A}(\mathbf{a}^{\dagger}) =  \mathbf{a}^{\dagger}) = P(\mathbf{W}= \mathbf{w}, \mathbf{A} =  \mathbf{a}^{\dagger}) $$
 
\end{lemma}

\begin{lemma}[Lemma 50 from \citetSM{Richardson2013}] \label{lemma50}

Given a DAG $\mathcal{G}$ let $T\in\mathbf{V}$ such that $ch_{\mathcal{G}}(T) = \emptyset$. Let $\mathbf{V}' = \mathbf{V}\setminus T$ and $\mathbf{V}'(\tilde{\mathbf{a}}) = \mathbf{V}'(\tilde{\mathbf{a}}) \setminus T(\tilde{\mathbf{a}})$. Further let $\mathcal{G}'=\mathcal{G}_{\mathbf{V}}$ and $\mathcal{G}'(\tilde{\mathbf{a}})=(\mathcal{G}(\tilde{\mathbf{a}}))_{\mathbb{V}'(\tilde{\mathbf{a}})\cup \tilde{\mathbf{a}}}$ be the reduced subgraphs obtained by removing $T$ and $T(\tilde{\mathbf{a}})$ from $\mathcal{G}$ and $\mathcal{G}(\tilde{\mathbf{a}})$. If $P(\mathbf{V})$ and $P(\mathbb{V}(\mathbf{a}^{\dagger}))$ factorize and obey modularity with respect to $\mathcal{G}$ and $\mathcal{G}(\tilde{\mathbf{a}})$ then $P(\mathbf{V}')$ and $P(\mathbb{V}'(\mathbf{a}^{\dagger}))$ factorize and obey modularity with respect to $\mathcal{G}'$ and $\mathcal{G}'(\tilde{\mathbf{a}'})$.
 
\end{lemma}

As shown in \citetSM{Richardson2013}, under a NPSEM associated with an FFRCISTG, the counterfactuals defined by Definition \ref{def: CEA} exist and have the independence structure defined by Definition \ref{def: FFRind}. Furthermore, when a graph is associated with an NPSEM in the usual way, the assumption of such an NPSEM implies factorization and modularity. Therefore, all subsequent results premised on factorization and modularity will follow under the causal model developed in the main text.

\subsection{Proof of the dynamic g-formula collapse}

\begin{definition}[Multivariate g-formulae] \label{def: mvgforms}
Define the full conditional g-formula $b^{\text{full}}_{\mathbf{a}^{\dagger}}(\mathbf{z}_m \mid \mathbf{\overline{h}}_m, \mathbf{\overline{l}}_m)$ and the full extended g-formula  $ f^{g}_{\text{full}}(\mathbf{z}) $ as

\begin{align*}
    b^{\text{full}}_{\mathbf{a}^{\dagger}}(\mathbf{z}_m \mid \mathbf{\overline{h}}_m, \mathbf{\overline{l}}_m)=  \sum\limits_{ \mathbf{\underline{h}}_{m+1}, \mathbf{s}_m}
        p(y\mid \mathbf{\overline{h}}_K, \mathbf{\overline{l}}_K, \mathbf{\overline{a}}_K^+)
        \prod\limits_{j=m+1}^{K}
        p(h_j, l_j, a_j \mid \mathbf{\overline{h}}_{j-1}, \mathbf{\overline{l}}_{j-1}, \mathbf{\overline{a}}_{j-1}^+),
\end{align*}

and 

\begin{align*}
   f^{g}_{\text{full}}(\mathbf{z}) =  \sum\limits_{\mathbf{a}^+, \mathbf{h}, \mathbf{s}}
        p(y\mid \mathbf{\overline{h}}_K, \mathbf{\overline{l}}_K, \mathbf{\overline{a}}_K^+)
        \prod\limits_{j=1}^{K}
        p(h_j, l_j, a_j \mid \mathbf{\overline{h}}_{j-1}, \mathbf{\overline{l}}_{j-1}, \mathbf{\overline{a}}_{j-1}^+)
        \prod\limits_{t=1}^{K}
        q_t^{g}(a_t^+ \mid \mathbf{pa}_t^+),
\end{align*}

and define the conditional g-formula $b_{\mathbf{a}^{\dagger}}(\mathbf{z}_m \mid \mathbf{\overline{l}}_m)$ and the extended dynamic g-formula  $f^{g}(\mathbf{z})$ as

\begin{align*}
    b_{\mathbf{a}^{\dagger}}(\mathbf{z}_m \mid  \mathbf{\overline{l}}_m)=  \sum\limits_{ \mathbf{s}_m}
        p(y\mid \mathbf{\overline{l}}_K, \mathbf{\overline{a}}_K^+)
        \prod\limits_{j=m+1}^{K}
        p(l_j, a_j \mid \mathbf{\overline{l}}_{j-1},\mathbf{\overline{a}}_{j-1}^+),
\end{align*}

and 

\begin{align*}
   f^{g}(\mathbf{z})=  \sum\limits_{\mathbf{a}^+,  \mathbf{s}}
        p(y\mid \mathbf{\overline{l}}_K, \mathbf{\overline{a}}_K^+)
        \prod\limits_{j=1}^{K}
        p(l_j, a_j \mid \mathbf{\overline{l}}_{j-1}, \mathbf{\overline{a}}_{j-1}^+)
        \prod\limits_{t=1}^{K}
        q_t^{g}(a_t^+ \mid \mathbf{pa}_t^+).
\end{align*}

Finally, define the reduced dynamic g-formula as:

\begin{align*}
   f^{g, \textbf{red}}(\mathbf{z'})=  \sum\limits_{\mathbf{a}^+,  \mathbf{s'}}
        p(y\mid \mathbf{\overline{l}'}_K, \mathbf{\overline{a}}_K^+)
        \prod\limits_{j=1}^{K}
        p(l'_j \mid \mathbf{\overline{l}'}_{j-1}, \mathbf{\overline{a}}_{j-1}^+)
        \prod\limits_{t=1}^{K}
        \tilde{q}_t^{g}(a_t^+ \mid \overline{l}'_{t}, \overline{a}_{t-1}^+).
\end{align*}

where $\tilde{q}_t^{g}$ are obtained recursively by: 

\begin{align*}
    \tilde{q}_t^{g}(a_t^+ \mid \overline{l}'_{t}, \overline{a}_{t-1}^+) = 
    \Bigg\{
        \prod\limits_{m=1}^{t-1} 
            \tilde{q}_m^{g}(a_t^+ \mid \overline{l}'_{m}, \overline{a}_{m-1}^+) 
    \Bigg\}^{-1}
    \Bigg\{ 
        \sum\limits_{\overline{r}_t, \overline{a}_t,}
        \prod\limits_{m=1}^{t} 
            q_m^{g}(a_m^+ \mid \text{pa}_m^+)p(a_m,r_m \mid \overline{l'}_{m}, \overline{a}_{m-1}^+)
    \Bigg\}.
\end{align*}

\end{definition}

\begin{lemma}[Lemma 58: Multivariate g-formula collapse, from \citetSM{Richardson2013}]\label{lemma: MVgcol}
Suppose $P(V)$ and $P(\mathbb{V}(\mathbf{a^{\dagger}}))$ obey modularity and factorize according to $\mathcal{G}$ and $\mathcal{G}(\mathbf{a^{\dagger}})$. The following independence conditions hold for $m=1,\dots,K$ for all $\mathbf{l}_m$

\begin{align} \label{eq: seqex}
    \mathbb{Z}_m(\mathbf{a^{\dagger}}) \CI I(A_m(\mathbf{a^{\dagger}}) = a^{\dagger}_m) \mid \overline{\mathbb{L}}_m(\mathbf{a^{\dagger}}) = \overline{\mathbf{l}}_m, \overline{\mathbb{A}}_{m-1}(\mathbf{a^{\dagger}}) = \overline{\mathbf{a}}^{\dagger}_{m-1}
\end{align}

if and only if for $m=1,\dots,K$ for all $\mathbf{l}_m$,

\begin{align}
       \sum\limits_{\mathbf{\overline{h}}_m}
        b^{\text{full}}_{\mathbf{a}^{\dagger}}(\mathbf{z}_m \mid \mathbf{\overline{h}}_m, \mathbf{\overline{l}}_m)
        p(\mathbf{\overline{h}}_m \mid \mathbf{\overline{l}}_m, \mathbf{\overline{a}}_{m-1}^{\dagger})
=       b_{\mathbf{a}^{\dagger}}(\mathbf{z}_m \mid \mathbf{\overline{l}}_m).
\end{align}\label{lem:rr58}
\end{lemma}

\begin{definition}\label{def: sub}
Define the regime $g_{-k}$ to be identical to the regime $g$, except the intervention on treatment at time $k$ is omitted, and the functions for assigning treatment at time $j>k$ are modified so that $A_j^{g+} = A_j^{g_{-k}+}$ whenever $A_k^{g+} = A_k^{g}$. Let  $\mathcal{G}(g_{-k})$ be its corresponding d-SWIG and $\mathcal{G}_(\mathbf{a}^{\dagger}_{-k})$ the static regime SWIG induced by the static intervention that sets $A\setminus A_k$ to $\mathbf{a}^{\dagger} \setminus \mathbf{a}^{\dagger}_k$.

\end{definition}

\begin{lemma} \label{lemma: irrel}
Suppose \eqref{eq: seqex} holds for $\mathbb{Z}(\mathbf{a}^{\dagger})$ defined with respect to regime $g$ at all time points $m=1,\ldots, k$. Suppose also that $A_k^{+}(g) \notin \text{anc}(Y(g))$. Then the following propositions hold for $m=1,\dots,k-1, k+1, \dots, K$ for all $\mathbf{l}_m$ and $a_k$:

\begin{align}
    \mathbb{Z}(g) = & \mathbb{Z}(g_{-k}) \label{eq: irrel1}\\
    \mathbb{Z}(\mathbf{a^{\dagger}}) = & \mathbb{Z}(\mathbf{a^{\dagger}_{-k}}) \label{eq: irrel2}\\
    \mathbb{Z}_m(\mathbf{a^{\dagger}_{-k}}) \CI & I(A_m(\mathbf{a^{\dagger}_{-k}}) = a^{\dagger}_m) \mid \overline{\mathbb{L}}_m(\mathbf{a^{\dagger}}_{-k}) = \overline{\mathbf{l}}_m,
    \{\overline{\mathbb{A}}_{m-1}(\mathbf{a^{\dagger}}_{-k}) \setminus A_k(\mathbf{a^{\dagger}}_{-k})\}  = \{\overline{\mathbf{a}}^{\dagger}_{m-1}\setminus a^{\dagger}_{k}\}
    \label{eq: irrel3}
\end{align}
\end{lemma}

\begin{proof}
\eqref{eq: irrel1} and \eqref{eq: irrel2} follow immediately by recursive substitution. Note that for $m<k$ \eqref{eq: irrel3} is equivalent to \eqref{eq: seqex} by recursive substitution and \eqref{eq: irrel2}. Now we prove  \eqref{eq: irrel3} by contradiction for $m>k$. Suppose for some $m>k$, \eqref{eq: irrel3} did not hold. Then it must be the case that 

\begin{align}\label{eq: irrel4}
    \mathbb{Z}_m(\mathbf{a^{\dagger}_{-k}}) \not\CI & I(A_k(\mathbf{a^{\dagger}_{-k}}) = a^{\dagger}_k) \mid \overline{\mathbb{L}}_k(\mathbf{a^{\dagger}}_{-k}) = \overline{\mathbf{l}}_k,
    \overline{\mathbb{A}}_{k-1}(\mathbf{a^{\dagger}}_{-k})  = \overline{\mathbf{a}}^{\dagger}_{k-1}.
\end{align}

As such either of the following must be true: there is an unblocked back-door path between $A_k(\mathbf{a^{\dagger}_{-k}})$ and $\mathbb{Z}_m(\mathbf{a^{\dagger}_{-k}})$ or there is a directed path between $A_k(\mathbf{a^{\dagger}_{-k}})$ and $\mathbb{Z}_m(\mathbf{a^{\dagger}_{-k}})$. The former implies a contradiction with \eqref{eq: seqex}, whereas the latter implies a contradiction with \eqref{eq: irrel2}. Therefore, \eqref{eq: irrel4} must NOT be the case and therefore if \eqref{eq: seqex} holds (the premise of the Lemma) then \eqref{eq: irrel3} must hold.
\end{proof}

\begin{lemma}[Lemma 59: Dynamic g-formula collapse from \citetSM{Richardson2013}]\label{lemma: Dyngcol}

Suppose the conditions of Lemma \ref{lemma: MVgcol} hold and also that the sequential independence conditions of expression \eqref{eq: seqex} hold for all $m$. Then,

$f^{g}_{\text{full}}(\mathbf{z}) = f^{g}(\mathbf{z})$.
\end{lemma}

\begin{proof}
Now we prove Lemma \ref{lemma: Dyngcol}. For compactness, we let $w_j \equiv \{h_j, l_j\}$ and first, we re-arrange terms:

\begin{align}
    f^{g}_{\text{full}}(\mathbf{z}) 
    = & \sum\limits_{\mathbf{a}^+, \mathbf{s}}\Bigg\{\prod\limits_{t=1}^{K}
        q_t^{g}(a_t^+ \mid \mathbf{pa}_t^+)\Bigg\}
        \sum\limits_{\mathbf{h}}p(y\mid \mathbf{\overline{w}}_K, \mathbf{\overline{a}}_K^+)
        \prod\limits_{j=1}^{K}
        p(w_j, a_j \mid \mathbf{\overline{w}}_{j-1}, \mathbf{\overline{a}}_{j-1}^+), \label{eq: intermed}
\end{align}

where the reformulation is justified because by definition $\mathbf{pa}_t^+ \cap \mathbf{h} = \emptyset$ for all $t$. 

Now we consider 2 cases, separately: (i) for all $t$, $A_{t}^+(g) \in \text{anc}(Y(g))$; and (ii) for all $t\neq k$, $A_{t}^+(g) \in \text{anc}(Y(g))$ but $A_{k}^+(g) \notin \mathbb{Z}(g)$.

Considering case (i), we re-write \eqref{eq: intermed} and apply Lemma \ref{lemma: MVgcol}: 

\begin{align*}
    f^{g}_{\text{full}}(\mathbf{z}) 
    = & \sum\limits_{\mathbf{a}^+, \mathbf{s}}\Bigg\{\prod\limits_{t=1}^{K}
        q_t^{g}(a_t^+ \mid \mathbf{pa}_t^+)\Bigg\}
        \sum\limits_{\mathbf{h}}p(y\mid \mathbf{\overline{w}}_K, \mathbf{\overline{a}}_K^+)
        \prod\limits_{j=1}^{K}
        p(w_j, a_j \mid \mathbf{\overline{w}}_{j-1}, \mathbf{\overline{a}}_{j-1}^+), \\
     = & \sum\limits_{\mathbf{a}^+}\Bigg\{\prod\limits_{t=1}^{K}
        q_t^{g}(a_t^+ \mid \mathbf{pa}_t^+)\Bigg\}\Bigg\{
        \sum\limits_{\mathbf{h},  \mathbf{s}}p(y\mid \mathbf{\overline{w}}_K, \mathbf{\overline{a}}_K^+)
        \prod\limits_{j=1}^{K}
        p(w_j, a_j \mid \mathbf{\overline{w}}_{j-1}, \mathbf{\overline{a}}_{j-1}^+)\Bigg\}, \\
    = & \sum\limits_{\mathbf{a}^+}\Bigg\{\prod\limits_{t=1}^{K}
        q_t^{g}(a_t^+ \mid \mathbf{pa}_t^+)\Bigg\}\Bigg\{\sum\limits_{l_1}\bigg[
        \sum\limits_{\mathbf{h_1}}b^{\text{full}}_{\mathbf{a}^{\dagger}}(\mathbf{z}_1 \mid h_1, l_1)
        p(h_1 \mid l_1)\bigg]p(l_1)\Bigg\}, \\
    = & \sum\limits_{\mathbf{a}^+}\Bigg\{\prod\limits_{t=1}^{K}
        q_t^{g}(a_t^+ \mid \mathbf{pa}_t^+)\Bigg\}\Bigg\{\sum\limits_{l_1}\bigg[
        b_{\mathbf{a}^{\dagger}}(\mathbf{z}_1 \mid  l_1)\bigg]p(l_1)\Bigg\}, \\
    = & \sum\limits_{\mathbf{a}^+}\Bigg\{\prod\limits_{t=1}^{K}
        q_t^{g}(a_t^+ \mid \mathbf{pa}_t^+)\Bigg\}
        b_{\mathbf{a}^{\dagger}}(\mathbf{z}), \\
    = & f^{g}(\mathbf{z}),
\end{align*}

where the second equality crucially follows because of by (i), then $\mathbf{pa}_t^+ \in \mathbf{z}$ for all $t$ and therefore $\mathbf{pa}_t^+ \notin \mathbf{s}$ for all $t$. The third equality follows by probability laws and the fourth equality holds by Lemma \ref{lem:rr58}.

Considering case (ii): by Lemma \ref{lemma: irrel}, Expression \eqref{eq: irrel1}, it follows immediately that $P(\mathbb{Z}(g) = \mathbf{z}) = P(\mathbb{Z}(g_{-k}) = \mathbf{z})$, and by \eqref{eq: irrel3}, then $P(\mathbb{Z}(g_{-k})=\mathbf{z}) = f^{g_{-k}}_{\text{full}}(\mathbf{z})$ which is given by Expression (\ref{eq: ii}) where we treat $A_k$ as a hidden variable in $\mathbf{H}$. Then it follows that $f^{g}_{\text{full}}(\mathbf{z}) = f^{g_{-k}}_{\text{full}}(\mathbf{z})$. Letting $\mathbf{\overline{a}}_{-k}^{\dagger} = \mathbf{\overline{a}}_{K}^{\dagger}\setminus a_k $:

\begin{align}
    f^{g}_{\text{full}}(\mathbf{z}) 
    = & \sum\limits_{\mathbf{a}^+, \mathbf{s}, \mathbf{h}}\Bigg\{\prod\limits_{t=1}^{K}
        q_t^{g}(a_t^+ \mid \mathbf{pa}_t^+)\Bigg\}
        \underbrace{p(y\mid \mathbf{\overline{w}}_K, \mathbf{\overline{a}}_K^+)
        \prod\limits_{j=1}^{K}
        p(w_j, a_j \mid \mathbf{\overline{w}}_{j-1}, \mathbf{\overline{a}}_{j-1}^+)}_{(\ast)}, \nonumber\\
 = & \sum\limits_{\mathbf{a}_{-k}^+, \mathbf{s}, \mathbf{h}}\Bigg\{\prod\limits_{t\neq k}
        q_t^{g}(a_t^+ \mid \mathbf{pa}_t^+)\Bigg\}
        p(y\mid \mathbf{\overline{w}}_K, \mathbf{\overline{a}}_{-k}^+)
        \begin{pmatrix*}[l]
         \prod\limits_{j=k+1}^{K} &
        p(w_j, a_j \mid \mathbf{\overline{w}}_{j-1}, \mathbf{a}_{j-1}^+, \dots, \mathbf{a}_{k+1}^+,a_k, \mathbf{\overline{a}}_{k-1}^+) \\
        \prod\limits_{j=1}^{k} &
        p(w_j, a_j \mid \mathbf{\overline{w}}_{j-1},  \mathbf{\overline{a}}_{j-1}^+) \\
        \end{pmatrix*} \label{eq: ii}\\
    = & \sum\limits_{\mathbf{a}_{K}^+, \mathbf{s}, \mathbf{h}}\
    \begin{Bmatrix*}[l]
    \prod\limits_{t=1}^K &
        q_t^{g}(a_t^+ \mid \mathbf{pa}_t^+) \\
    \end{Bmatrix*}
        p(y\mid \mathbf{\overline{w}}_K, \mathbf{\overline{a}}_{-k}^+)
        \begin{pmatrix*}[l]
         \prod\limits_{j=k+1}^{K} &
        p(w_j, a_j \mid \mathbf{\overline{w}}_{j-1}, \mathbf{a}_{j-1}^+, \dots, \mathbf{a}_{k+1}^+, a_k, \mathbf{\overline{a}}_{k-1}^+) \\
        \prod\limits_{j=1}^{k} &
        p(w_j, a_j \mid \mathbf{\overline{w}}_{j-1},  \mathbf{\overline{a}}_{j-1}^+)
        \end{pmatrix*}
         \nonumber
\end{align}

where the second equality expresses the equality $f^{g}_{\text{full}}(\mathbf{z}) = f^{g_{-k}}_{\text{full}}(\mathbf{z})$. The third follows because, for each $\mathbf{s}$, we can additionally sum over $a_k^{+}$ because all the other terms are not a function of  $a_k^{+}$ and $\sum\limits_{\mathbf{a}_{k}^+}q_k^{g}(a_k^+ \mid \mathbf{pa}_k^+)=1$. Then we can see that $(*)$ under case (ii) is not actually a function of $a^{+}_k$.

Then consider the set $\mathbf{s}$ and note $\mathbf{s}\not\in \{\mathbf{pa}_t^+ \mid t>k\}$ because by supposition $\{\mathbf{pa}_t^+ \mid t>k\} \subseteq z$. Therefore, we can can continue the panel from expression \eqref{eq: ii} and write: 
\begin{align}
    = & \sum\limits_{\mathbf{a}_{-k}^+}\
    \underbrace{\begin{Bmatrix*}[l]
    \prod\limits_{t\neq k} 
        q_t^{g}(a_t^+ \mid \mathbf{pa}_t^+) \\
    \end{Bmatrix*}}_{(\ast\ast)}
    \sum\limits_{ \mathbf{s}, \mathbf{h}}
        p(y\mid \mathbf{\overline{w}}_K, \mathbf{\overline{a}}_{-k}^+)
        \begin{pmatrix*}[l]
         \prod\limits_{j=k+1}^{K} &
        p(w_j, a_j \mid \mathbf{\overline{w}}_{j-1}, \mathbf{a}_{j-1}^+, \dots, \mathbf{a}_{k+1}^+,a_k, \mathbf{\overline{a}}_{k-1}^+) \\
        \prod\limits_{j=1}^{k} &
        p(w_j, a_j \mid \mathbf{\overline{w}}_{j-1},  \mathbf{\overline{a}}_{j-1}^+)
        \end{pmatrix*} \label{eq: iia} \\ 
    = & \sum\limits_{\mathbf{a}_{-k}^+}
    \begin{Bmatrix*}[l]
    \prod\limits_{t\neq k}
        q_t^{g}(a_t^+ \mid \mathbf{pa}_t^+) \\
    \end{Bmatrix*}
    \begin{pmatrix*}[l]
    \sum\limits_{ l_1, h_1}
        P(\mathbb{Z}(\mathbf{a}_{-k}^{\dagger})= \mathbf{z} \mid h_1, l_1)p(h_1 \mid l_1)p(l_1)
        \end{pmatrix*}
          \nonumber \\
    = & \sum\limits_{\mathbf{a}_{-k}^+}
    \begin{Bmatrix*}[l]
    \prod\limits_{t\neq k}
        q_t^{g}(a_t^+ \mid \mathbf{pa}_t^+) \\
    \end{Bmatrix*}
    \begin{pmatrix*}[l]
    \sum\limits_{ l_1, h_1}
        P(\mathbb{Z}(\mathbf{a}^{\dagger})= \mathbf{z} \mid h_1, l_1)p(h_1 \mid l_1)p(l_1)
    \end{pmatrix*} \nonumber\\
    = &\sum\limits_{\mathbf{a}_{-k}^+, \mathbf{s}}
    \begin{Bmatrix*}[l]
    \prod\limits_{t\neq k}
        q_t^{g}(a_t^+ \mid \mathbf{pa}_t^+) \\
    \end{Bmatrix*}
        \underbrace{\Bigg\{
        p(y\mid \mathbf{\overline{l}}_K, \mathbf{\overline{a}}_K^+)
        \prod\limits_{j=1}^{K}
        p(l_j, a_j \mid \mathbf{\overline{l}}_{j-1}, \mathbf{\overline{a}}_{j-1}^+)\Bigg\}}_{(\ast)} \nonumber\\
    = &\sum\limits_{\mathbf{a}_{K}^+, \mathbf{s}}
    \begin{Bmatrix*}[l]
    \prod\limits_{t=1}^{K}
        q_t^{g}(a_t^+ \mid \mathbf{pa}_t^+) \\
    \end{Bmatrix*}
        \Bigg\{
        p(y\mid \mathbf{\overline{l}}_K, \mathbf{\overline{a}}_K^+)
        \prod\limits_{j=1}^{K}
        p(l_j, a_j \mid \mathbf{\overline{l}}_{j-1}, \mathbf{\overline{a}}_{j-1}^+)\Bigg\} \nonumber\\
    = & f^{g}(\mathbf{z}) \nonumber
\end{align}

The second equality follows by factorisation and modularity, the third by Lemma \ref{lemma: irrel}, the fourth by the same arguments used in the proof for case $(i)$, the fifth by the same arguments justifying the equality in expression \eqref{eq: iia}, the sixth by previous arguments that none of the terms in $(\ast\ast)$ or $(\ast)$ are functions of $a_k^+$, and the last by definition of the dynamic g-formula.

To generalize, consider the set of indices $\mathcal{J} \subseteq \{1,\dots, K\}$. Then consider regimes $g_{-\mathcal{J}}$ to be those analogous to $g_{-k}$ except removing intervention on \textit{all} treatments indexed by values in $\mathcal{J}$. Then consider analogue to Lemma \ref{lemma: irrel} and repeat the preceding analysis with the more general treatment node-set. This completes the proof because cases (i) and (ii) cover the space of possible circumstances, when considering treatments $\mathcal{J}$ instead of $k$.

\end{proof}
