# Supplementary material for: Interpretational errors in statistical causal inference
Source: arXiv:2312.07610 source file (2023-12-11)
Supplement: Supplementary file 2 [file AppendixB_ProofRedGform.tex]

%\begin{definition}[Relevant Instruments] 
%Define the set of relevant natural treatment values $a\subseteq A$ and relevant time-varying instruments $r\subseteq R$ as those that are ancestors of $Y$ under regime $g$ (and are thus necessarily used to assign treatment under regime $g$). Denote their respective complements (the irrelevant natural values of treatment and instruments) by $A'$ and $R'$.

%\begin{align*}
%    \mathbb{A}^{*}(g) & \equiv \mathbb{R}(g) \cap \mathbb{Z}(g) \\
%    \mathbb{R}^{*}(g) & \equiv \mathbb{R}(g) \cap \mathbb{Z}(g) \\
%    \mathbb{A}^{'}(g) & \equiv \mathbb{R}(g) \setminus \mathbb{A}^*(g) \\
%    \mathbb{R}^{'}(g) & \equiv \mathbb{R}(g) \setminus \mathbb{r}(g) \\.
%\end{align*}
%. 
%\end{definition}

\subsection{Proof of Theorem \ref{thm: stochgform}, and related results}
 
\subsubsection{Supporting Lemmas and their proofs}
 
\begin{lemma}[Treatment exchangeability under extended regime]
Consider a model in which the conditions of Lemma \ref{lemma: Dyngcol} (Dynamic g-formula collapse) hold, and consider the set of time-varying instruments defined as in Definition \ref{def: TVI}. Then the following exchangeability condition holds:

\begin{align}
    & \mathbb{Z}_{m}(\mathbf{a^{\dagger}}, \mathbf{r}^{\dagger} ) \CI   I(\mathbb{A}_m(\mathbf{a^{\dagger}}, \mathbf{r}^{\dagger}) = \mathbf{a^{\dagger}}_m) \Big|  \overline{\mathbb{L}}_m(\mathbf{a}^{\dagger}, \mathbf{r}^{\dagger}), \overline{\mathbb{A}}_{m-1}(\mathbf{a}^{\dagger}, \mathbf{r}^{\dagger}). \label{eq: irrel2RA}   
\end{align}

\end{lemma}

\begin{proof}
Exchangeability condition \eqref{eq: seqex} implies 

\begin{align*} 
    \mathbb{Z}_m(\mathbf{a^{\dagger}}) \CI I(\mathbb{A}_m(\mathbf{a^{\dagger}}) = a^{\dagger}_m) \mid \overline{\mathbb{L}}_m(\mathbf{a^{\dagger}}) = \{\overline{\mathbf{r}}_m^{\dagger}, \overline{\mathbf{l}}'_m\} , \overline{\mathbb{A}}_{m-1}(\mathbf{a^{\dagger}}) = \overline{\mathbf{a}}^{\dagger}_{m-1}.
\end{align*}

Applying Lemma \ref{lemma49} (consistency) then provides the result.

\end{proof}

\begin{lemma} [Incomplete collision for non-ancestors]  \label{lemma: indgenlemma}
Consider a regime $g$ that intervenes on $A$. Consider a model in which the conditions of Lemma \ref{lemma: Dyngcol} (Dynamic g-formula collapse) hold and let $R$ be the set of time-varying instruments for $A$ with respect to $Z$ (defined relative to regime $g$ as in definition \ref{def: Zset}). Suppose also that for each $j$, $S^{'*}_j$ is a confounder so that there exists the path $S^{'*}_j\leftarrow \circ \rightarrow Z_j$, or else is $\emptyset$.

Then the following propositions hold. First, for each $k$, at least one of the two conditions $(i)$ or $(ii)$ holds for all $j<k$:

\begin{itemize}
    \item [$(i)$] 
    \begin{align}
    \mathbb{R}_k (\mathbf{a^{\dagger}}, \mathbf{r})
        \CI 
            \mathbb{S}^{'*}_{j}(\mathbf{a^{\dagger}}, \mathbf{r})
        \mid
            \overline{\mathbb{Z}}^{'*}_{k}(\mathbf{a^{\dagger}}, \mathbf{r}), 
            \overline{\mathbb{S}}^{'*}_{j-1}(\mathbf{a^{\dagger}}, \mathbf{r}),
            \overline{\mathbb{A}}_{j-1}(\mathbf{a^{\dagger}}, \mathbf{r}),
            \overline{\mathbb{R}}_{j-1}(\mathbf{a^{\dagger}}, \mathbf{r}),
            \label{eq: indgenlemma1}
    \end{align}
    \item [$(ii)$] 
    \begin{align}
    \mathbb{Z}_k (\mathbf{a^{\dagger}}, \mathbf{r})
        \CI 
            \mathbb{S}^{'*}_{j}(\mathbf{a^{\dagger}}, \mathbf{r})
        \mid
            \overline{\mathbb{Z}}^{'*}_{k}(\mathbf{a^{\dagger}}, \mathbf{r}), 
            \overline{\mathbb{S}}^{'*}_{j-1}(\mathbf{a^{\dagger}}, \mathbf{r}),
            \overline{\mathbb{A}}_{j-1}(\mathbf{a^{\dagger}}, \mathbf{r}),
            \overline{\mathbb{R}}_{j-1}(\mathbf{a^{\dagger}}, \mathbf{r}).
            \label{eq: indgenlemma2}
    \end{align}
\end{itemize}

Furthermore, the above proposition holds, except replacing $\Big(\mathbb{A}_k (\mathbf{a^{\dagger}}, \mathbf{r}), \mathbb{R}_k (\mathbf{a^{\dagger}}, \mathbf{r})\Big)$ in place of $\mathbb{R}_k (\mathbf{a^{\dagger}}, \mathbf{r})$ in \eqref{eq: indgenlemma1}.

Second, for each $k$, the following proposition holds:

\begin{align}
    \mathbb{R}_k (\mathbf{a^{\dagger}}, \mathbf{r})
        \CI 
            \mathbb{S}^{'*}_{k}(\mathbf{a^{\dagger}}, \mathbf{r})
        \mid
            \overline{\mathbb{Z}}^{'*}_{k}(\mathbf{a^{\dagger}}, \mathbf{r}), 
            \overline{\mathbb{S}}^{'*}_{k-1}(\mathbf{a^{\dagger}}, \mathbf{r}),
            \overline{\mathbb{A}}_{k-1}(\mathbf{a^{\dagger}}, \mathbf{r}),
            \overline{\mathbb{R}}_{k-1}(\mathbf{a^{\dagger}}, \mathbf{r}),
            \label{eq: indgenlemma3}
    \end{align}
\end{lemma}

Furthermore, the above proposition holds, except replacing $\Big(\mathbb{A}_k (\mathbf{a^{\dagger}}, \mathbf{r}), \mathbb{R}_k (\mathbf{a^{\dagger}}, \mathbf{r})\Big)$ in place of $\mathbb{R}_k (\mathbf{a^{\dagger}}, \mathbf{r})$ in \eqref{eq: indgenlemma3}.

\begin{proof}
To prove Lemma \ref{lemma: indgenlemma} we consider proof for contradiction. 

First, suppose \eqref{eq: indgenlemma1} does not hold. Note that, since $R_k\in Z$, there cannot exist any directed path $S^{'*}_j \rightarrow \circ \rightarrow \cdots \rightarrow R_k$, where $\circ$ represents some nodes in $\{U, S\}$, otherwise, $S^{'*}_j\in Z$. Therefore there must exist one of the two following paths (where $\circ$ represents unmeasured nodes and $\ast$ represent colliders in $\{\mathbf{\overline{Z}}^{'*}_{k}, \mathbf{\overline{S}}^{'*}_{j-1}, \mathbf{\overline{A}}_{j-1}, \mathbf{\overline{R}}_{j-1} \}$):

\begin{itemize}
    \item [$(ia)$] $S^{'*}_j \leftarrow \circ \rightarrow  R_k$, or
    \item [$(ib)$] $S^{'*}_j \leftarrow \circ \rightarrow  \ast \leftarrow \circ \rightarrow \ast \leftarrow \cdots \rightarrow  \ast \leftarrow \circ \rightarrow R_k$.
\end{itemize}

Second, suppose \eqref{eq: indgenlemma2} does not hold. Note again that there cannot exist any directed path $S^{'*}_j \rightarrow \circ \rightarrow \cdots \rightarrow Z_k$, where $\circ$ represents some nodes in $\{U, S\}$, otherwise, $S^{'*}_j\in Z$. Therefore there must exist one of the two following paths:

\begin{itemize}
    \item [$(iia)$] $S^{'*}_j \leftarrow \circ \rightarrow  Z_k$, or
    \item [$(iib)$] $S^{'*}_j \leftarrow \circ \rightarrow  \ast \leftarrow \circ \rightarrow \ast \leftarrow \cdots \rightarrow  \ast \leftarrow \circ \rightarrow Z_k$.
\end{itemize}

Now suppose at least one of $\{(ia), (ib)\}$ holds and at least one of $\{(iia), (iib)\}$ holds. Then at least one of the following paths exists:

\begin{itemize}
    \item [$(ia) + (iia)$] $R_k \leftarrow \circ \rightarrow S^{'*}_j \leftarrow \circ \rightarrow  Z_k$ or 
    \item [$(ia) + (iib)$] $R_k \leftarrow \circ \rightarrow S^{'*}_j \leftarrow \circ \rightarrow  \ast \leftarrow \circ \rightarrow \ast \leftarrow \cdots \rightarrow  \ast \leftarrow \circ \rightarrow Z_k$ or 
    \item [$(ib) + (iia)$] $R_k \leftarrow \circ \rightarrow  \ast \leftarrow \circ \rightarrow \ast \leftarrow \cdots \rightarrow  \ast \leftarrow \circ \rightarrow S^{'*}_j \leftarrow \circ \rightarrow  Z_k$ or 
    \item [$(ib) + (iib)$] $R_k \leftarrow \circ \rightarrow  \ast \leftarrow \circ \rightarrow \ast \leftarrow \cdots \rightarrow  \ast \leftarrow \circ \rightarrow S^{'*}_j \leftarrow \circ \rightarrow  \ast \leftarrow \circ \rightarrow \ast \leftarrow \cdots \rightarrow  \ast \leftarrow \circ \rightarrow Z_k$.
\end{itemize}

But each of these paths would contradict condition \eqref{eq: irrel2R} (sequential exchangeability for the instrument): all of the variables in $*$, $\{\mathbf{\overline{Z}}^{'*}_{k}, \mathbf{\overline{S}}^{'*}_{j-1}, \mathbf{\overline{A}}_{j-1}, \mathbf{\overline{R}}_{j-1} \}$, are in the conditioning event of the independence of expression \eqref{eq: irrel2R}. Therefore, if not $(i)$ then $(ii)$ and if not $(ii)$ then $(i)$. Identical arguments are used to justify the case for $\{A_k, R_k\}\in Z$.

To prove condition \eqref{eq: indgenlemma3}, note again that for it not to hold, then either $(ia)$ or $(ib)$ must hold, taking $j=k$. But by supposition, we also have $S^{'*}_k\leftarrow \circ \rightarrow Z_k$. So if condition \eqref{eq: indgenlemma3} does not hold then we will have one of the following paths:

\begin{itemize}
    \item [$(ia)$] $R_k \leftarrow \circ \rightarrow S^{'*}_k \leftarrow \circ \rightarrow  Z_k$ or 
    \item [$(ib)$] $R_k \leftarrow \circ \rightarrow  \ast \leftarrow \circ \rightarrow \ast \leftarrow \cdots \rightarrow  \ast \leftarrow \circ \rightarrow S^{'*}_k \leftarrow \circ \rightarrow  Z_k$.
\end{itemize}

But each of these paths would again contradict condition \eqref{eq: irrel2R} (sequential exchangeability for the instrument). For the case with $\{A_k, R_k\}$, the independence will hold trivially because then $S^{'*}_k$ could not be a confounder for $A_k$ -- if it were a cause of $A_k$ then it would be in $Z$ (a contradiction) and if it was associated with $A_k$ via some unmeasured cause $\circ$, then we would have the collider path $A_k \leftarrow \circ \rightarrow   S^{'*}_k \leftarrow \circ \rightarrow  Z_k$, which would contradict sequential exchangeability condition \eqref{eq: seqex}.
\end{proof}

\begin{lemma}[Collision impossibility for outcome ancestors]\label{lemma: indgenlemma2}
Consider a regime $g$ that intervenes on $A$. Consider a model in which the conditions of Lemma \ref{lemma: Dyngcol} (Dynamic g-formula collapse) hold and let $R$ be the set of time-varying instruments for $A$ with respect to $Z$ (defined relative to regime $g$ as in definition \ref{def: Zset}). Suppose also that for each $j$, $S^{'*}_j$ is a confounder so that there exists the path $S^{'*}_j\leftarrow \circ \rightarrow Z_j$.

%Then, for each $k$, for all $j, p, s$ such that $k > j \geq p$ and $k>s$, 

%\begin{align}
%    \mathbb{Z}^{'*}_k (\mathbf{a^{\dagger}}, \mathbf{r})
%        \CI 
%           \Big(\mathbb{A}_{j}(\mathbf{a^{\dagger}}, \mathbf{r}), %\mathbb{r}_{j}(\mathbf{a^{\dagger}}, \mathbf{r})\Big)
%        \mid
%            \overline{\mathbb{Z}}^{'*}_{k-1}(\mathbf{a^{\dagger}}, \mathbf{r}), 
%            \overline{\mathbb{S}}^{'*}_{p}(\mathbf{a^{\dagger}}, \mathbf{r}),
%            \overline{\mathbb{A}}_{s}(\mathbf{a^{\dagger}}, \mathbf{r}),
%            \overline{\mathbb{r}}_{j-1}(\mathbf{a^{\dagger}}, \mathbf{r}),
%            \label{eq: indgenlemma4}
%    \end{align}
%    
%and 
%
%\begin{align}
%    \mathbb{r}_k (\mathbf{a^{\dagger}}, \mathbf{r})
%        \CI 
%            \Big(\mathbb{A}_{j}(\mathbf{a^{\dagger}}, \mathbf{r}),
%            \mathbb{r}_{j}(\mathbf{a^{\dagger}}, \mathbf{r})\Big)
%        \mid
%            \overline{\mathbb{Z}}^{'*}_{k}(\mathbf{a^{\dagger}}, \mathbf{r}), 
%            \overline{\mathbb{S}}^{'*}_{p}(\mathbf{a^{\dagger}}, \mathbf{r}),
%            \overline{\mathbb{A}}_{s}(\mathbf{a^{\dagger}}, \mathbf{r}),
%            \overline{\mathbb{r}}_{j-1}(\mathbf{a^{\dagger}}, \mathbf{r}),
%            \label{eq: indgenlemma5}
%    \end{align}

Then, for each $k$, for all $j$ such that $j<k$, 

\begin{align}
    \mathbb{Z}^{'*}_{k} (\mathbf{a^{\dagger}}, \mathbf{r})
        \CI 
           \Big(\mathbb{A}_{j}(\mathbf{a^{\dagger}}, \mathbf{r}), \mathbb{R}_{j}(\mathbf{a^{\dagger}}, \mathbf{r})\Big)
        \mid
            \overline{\mathbb{Z}}^{'*}_{k-1}(\mathbf{a^{\dagger}}, \mathbf{r}), 
            \overline{\mathbb{S}}^{'*}_{j}(\mathbf{a^{\dagger}}, \mathbf{r}),
            \overline{\mathbb{A}}_{j-1}(\mathbf{a^{\dagger}}, \mathbf{r}),
            \overline{\mathbb{R}}_{j-1}(\mathbf{a^{\dagger}}, \mathbf{r}),
            \label{eq: indgenlemma4}
    \end{align}
    
and 

\begin{align}
    \Big(\mathbb{A}_k (\mathbf{a^{\dagger}}, \mathbf{r}), \mathbb{R}_k (\mathbf{a^{\dagger}}, \mathbf{r})\Big)
        \CI 
            \Big(\mathbb{A}_{j}(\mathbf{a^{\dagger}}, \mathbf{r}),
            \mathbb{R}_{j}(\mathbf{a^{\dagger}}, \mathbf{r})\Big)
        \mid
            \overline{\mathbb{Z}}^{'*}_{k}(\mathbf{a^{\dagger}}, \mathbf{r}), 
            \overline{\mathbb{S}}^{'*}_{j}(\mathbf{a^{\dagger}}, \mathbf{r}),
            \overline{\mathbb{A}}_{j-1}(\mathbf{a^{\dagger}}, \mathbf{r}),
            \overline{\mathbb{R}}_{j-1}(\mathbf{a^{\dagger}}, \mathbf{r}),
            \label{eq: indgenlemma5}
    \end{align}
\end{lemma}

\begin{proof}
Suppose the premises of Lemma \ref{lemma: indgenlemma2} held but \eqref{eq: indgenlemma4} did not. Then there must be some collider path of the following form:

$$\{R_j, A_j\} \leftarrow \circ \rightarrow  \ast \leftarrow \circ \rightarrow \ast \leftarrow \cdots \rightarrow  \ast \leftarrow \circ \rightarrow Z^{'*}_k,$$

 where $\circ$ represents unmeasured nodes and $\ast$ represent colliders in $\{Z^{'*}_{k-1},\dots, Z^{'*}_{j+1}\}$. But then there would exist the sub-path

 $$\{R_j, A_j\} \leftarrow \circ \rightarrow  \ast,$$ which would contradict the sequential exchangeabilities of conditions \eqref{eq: seqex} and \eqref{eq: irrel2R} . 
 
 The same arguments are use to justify \eqref{eq: indgenlemma5}.
 
\end{proof}

\begin{lemma}[Reduced exchangeability for relevant instruments]\label{lemma: rstarex}
Consider a regime $g$ that intervenes on $A$. Consider a model in which the conditions of Lemma \ref{lemma: Dyngcol} (Dynamic g-formula collapse) hold and let $R$ be the set of time-varying instruments for $A$ with respect to $Z$ (defined relative to regime $g$ as in definition \ref{def: Zset}). Consider the set of relevant instruments $R$. Then the reduced set of sequential exchangeability conditions hold:

\begin{align}
   & \mathbb{Z}_{m}(\mathbf{a^{\dagger}}, \mathbf{r}^{\dagger} ) \CI   \mathbb{R}_m(\mathbf{a^{\dagger}}, \mathbf{r}^{\dagger}) \Big|  \overline{\mathbb{Z}}^{'*}_m(\mathbf{a}^{\dagger}, \mathbf{r}^{\dagger}),  \overline{\mathbb{R}}_{m-1}(\mathbf{a}^{\dagger}, \mathbf{r}^{\dagger}). \label{eq: irrel2Rc}
\end{align}
\end{lemma}

\begin{proof}
Note that $R_j \in Z$. For $\overline{S}^{'*}_j$ to be a relevant confounder for $R_m$, then it must either be cause of $R_j$ or of some element in $\mathbb{Z}_{m}$. But then $\overline{S}^{'*}_j$ would contain an ancestor of $Y$ under $g$, which contradicts the definition of $\overline{S}^{'*}_j$.
\end{proof}

\subsubsection{Proof of Theorem \ref{thm: stochgform}}

Now we prove Theorem \ref{thm: stochgform}, where we consider, without loss of generality, the case where $\mathbb{A}^{g+} \subset an(Y(g))$, so that assigned treatment at each time point is a cause of the outcome under regime $g$. Furthermore, we consider the following condition to be the case, without loss of generality: each $S^{'*}_k $ is a parent of some treatment node $A_m$, with $m\geq k$ and that there exists some confounding path $S^{'*}_k \leftarrow \circ \rightarrow Z_k$, or else $S^{'*}_k$ would not be necessary to control for confounding and thus would be marginalized out of $\sum\limits_{\mathbf{a}, \mathbf{r}} P(\mathbb{Z}(g) = \mathbf{z})$ trivially.% according to arguments in Lemma \ref{lemma: redgform2} (Dynamic g-formula collapse over irrelevant instruments). 

For compactness, we write $p$, $p_{\mathbf{a^{\dagger}}}$, and $p_{\mathbf{a^{+}, \mathbf{r}}}$ to denote, respectively, densities of $V$, $\mathbb{V}(\mathbf{a^{+}})$, and $\mathbb{V}(\mathbf{a^{+}}, \mathbf{r})$.

Finally, whenever we consider densities for $\{a_j, r_j\}$, the natural value of treatment, and an instrument at time $j$ we will assume that each is an argument in the dynamic regime for some future \textit{assigned} value of treatment $a_m^+$, with $m\geq j$, otherwise each would be marginalized out of the g-formula trivially when summing over $\{a_j, r_j\}$.%, following arguments in Lemma \ref{lemma: redgform2} (Dynamic g-formula collapse over irrelevant instruments). Thus we will only consider terms with $\{a_j, r_j\}$

First we prove an intermediate Lemma:

\begin{lemma}\label{lemma: mainlemma}
Consider a regime $g$ that intervenes on $A$. Consider a model in which the conditions of Lemma \ref{lemma: Dyngcol} (Dynamic g-formula collapse) hold and let $R$ be the set of time-varying instruments for $A$ with respect to $Z$ (defined relative to regime $g$ as in definition \ref{def: Zset}). Then the following equality holds:

\begin{align}
\sum\limits_{\mathbf{a}', \mathbf{r}'} p_{\mathbf{a}^+}( \mathbf{z}) =
p_{\mathbf{a}^+}(y, \underline{\mathbf{z}}^{'*}_1) \prod\limits_{m=1}^{K}   
 p_{\mathbf{a}^+}(a_m, r_{m} \mid
                     \mathbf{\overline{z}}^{'*}_{m}, \mathbf{\overline{r}}_{m-1})  \label{eq: mainlemma}
\end{align}
\end{lemma}

\begin{proof}

First we note by the multivariate g-formula collapse Lemma \ref{lemma: MVgcol} that we can write the left-hand side of \eqref{eq: mainlemma} as follows:

\begin{align*}
\sum\limits_{s^{'*}_{1}} & 
         \begin{pmatrix*}[l] 
     &   p(a_{1}, r_{1} \mid
                     \mathbf{\overline{z}}^{'*}_{1},
                     \mathbf{\overline{s}}^{'*}_{1}) \\
         &   p(z^{'*}_{1} \mid 
                     s^{'*}_{1})   \\
         &  p(s^{'*}_{1} ) \\ 
        & \vdots \\
&    \cdots 
   \sum\limits_{s^{'*}_{m}}  
         \begin{pmatrix*}[l] 
         &   p(a_{m}, r_{m} \mid
                     \mathbf{\overline{z}}^{'*}_{m},
                     \mathbf{\overline{s}}^{'*}_{m},
                     \mathbf{\overline{a}}_{m-1}^+,
                     \mathbf{\overline{r}}_{m-1}) \\
         &   p(z^{'*}_{m} \mid 
                     \mathbf{\overline{s}}^{'*}_{m},
                     \mathbf{\overline{a}}_{m-1}^+,
                     \mathbf{\overline{r}}_{m-1}, 
                     \mathbf{\overline{z}}^{'*}_{m-1})   \\
         &  p(s^{'*}_{m} \mid 
                     \mathbf{\overline{a}}_{m-1}^+,
                     \mathbf{\overline{r}}_{m-1}, 
                     \mathbf{\overline{z}}^{'*}_{m-1},
                     \mathbf{\overline{s}}^{'*}_{m-1}) \\
       &  \vdots \\
 & \cdots  \sum\limits_{s^{'*}_{K}}                
            \begin{pmatrix*}[l]
                 &   p(y \mid 
                            \mathbf{\overline{a}}_{K}^+, 
                            \mathbf{\overline{r}}_{K}, 
                            \mathbf{\overline{z}}^{'*}_{K}, 
                            \mathbf{\overline{s}}^{'*}_{K}) \\
                 &   p(a_K, r_K \mid
                             \mathbf{\overline{z}}^{'*}_{K},
                             \mathbf{\overline{s}}^{'*}_{K},
                             \mathbf{\overline{a}}_{K-1}^+,
                             \mathbf{\overline{r}}_{K-1}) \\
                 &   p(z^{'*}_{K} \mid 
                             \mathbf{\overline{s}}^{'*}_{K},
                             \mathbf{\overline{a}}_{K-1}^+,
                             \mathbf{\overline{r}}_{K-1}, 
                             \mathbf{\overline{z}}^{'*}_{K-1})   \\
                 &  p(s^{'*}_{K} \mid 
                             \mathbf{\overline{a}}_{K-1}^+
                             \mathbf{\overline{r}}_{K-1}, 
                             \mathbf{\overline{z}}^{'*}_{K-1},
                             \mathbf{\overline{s}}^{'*}_{K-1}) 
            \end{pmatrix*}
\cdots
\end{pmatrix*}
\cdots
\end{pmatrix*}
\end{align*}

%$q_t$ in place of $q_t(a_t^+ \mid \mathbf{pa}_t^+)$. We also use 

Then we prove the equality in \eqref{eq: mainlemma} by focusing on the following equality and inducting on $m$:

\begin{align*}
 p_{\mathbf{a}^+}( \mathbf{z}) =
    \sum\limits_{s^{'*}_{1}} & 
         \begin{pmatrix*}[l] 
     &   p(a_{1}, r_{1} \mid
                     \mathbf{\overline{z}}^{'*}_{1},
                     \mathbf{\overline{s}}^{'*}_{1}) \\
         &   p(z^{'*}_{1} \mid 
                     s^{'*}_{1})   \\
         &  p(s^{'*}_{1} ) \\ 
        & \vdots \\
&    \cdots  \sum\limits_{s^{'*}_{m-1}}  \begin{pmatrix*}[l] 
&   p_{\mathbf{a}^+, \mathbf{r}}(y, \underline{\mathbf{z}}^{'*}_m \mid 
                     \mathbf{\overline{a}}_{m-1}^+,
                     \mathbf{\overline{r}}_{m-2}, 
                     \mathbf{\overline{z}}^{'*}_{m-1},
                     \mathbf{\overline{s}}^{'*}_{m-1}) \\
\prod\limits_{j=m}^{K}  & 
 p_{\mathbf{a}^+, \mathbf{r}}(a_{j}, r_{j} \mid
                     \mathbf{\overline{z}}^{'*}_{j},
                     \mathbf{\overline{s}}^{'*}_{m-1},
                     \mathbf{\overline{a}}_{j-1}^+,
                     \mathbf{\overline{r}}_{m-2})  
\end{pmatrix*}
\end{pmatrix*}.
\end{align*}

\underline{\textbf{The base case:}} First we prove the claim for the base case $m=K$ and also for $m=K-1$ and  $K-2$, to demonstrate arguments used for the inductive step.

Consider time point $K$:

\begin{align*}
       \sum\limits_{s^{'*}_{K}} &               
            \begin{Bmatrix*}[l]
                 &   p(y \mid 
                            \mathbf{\overline{a}}_{K}^+, 
                            \mathbf{\overline{r}}_{K}, 
                            \mathbf{\overline{z}}^{'*}_{K}, 
                            \mathbf{\overline{s}}^{'*}_{K}) \\
                 &   p(a_K, r_K \mid
                             \mathbf{\overline{z}}^{'*}_{K},
                             \mathbf{\overline{s}}^{'*}_{K},
                             \mathbf{\overline{a}}_{K-1}^+,
                             \mathbf{\overline{r}}_{K-1}) \\
                 &   p(z^{'*}_{K} \mid 
                             \mathbf{\overline{s}}^{'*}_{K},
                             \mathbf{\overline{a}}_{K-1}^+,
                             \mathbf{\overline{r}}_{K-1}, 
                             \mathbf{\overline{z}}^{'*}_{K-1})   \\
                 &  p(s^{'*}_{K} \mid 
                             \mathbf{\overline{a}}_{K-1}^+
                             \mathbf{\overline{r}}_{K-1}, 
                             \mathbf{\overline{z}}^{'*}_{K-1},
                             \mathbf{\overline{s}}^{'*}_{K-1}) 
            \end{Bmatrix*} \\
= 
       \sum\limits_{s^{'*}_{K}} &               
            \begin{Bmatrix*}[l]
                 &   p_{\mathbf{a}^+, \mathbf{r}}(y \mid 
                            \mathbf{\overline{a}}_{K}^+, 
                            \mathbf{\overline{r}}_{K}, 
                            \mathbf{\overline{z}}^{'*}_{K}, 
                            \mathbf{\overline{s}}^{'*}_{K}) \\
                 &   p_{\mathbf{a}^+, \mathbf{r}}(a_K, r_K \mid
                             \mathbf{\overline{z}}^{'*}_{K},
                             \mathbf{\overline{s}}^{'*}_{K},
                             \mathbf{\overline{a}}_{K-1}^+,
                             \mathbf{\overline{r}}_{K-1}) \\
                 &   p_{\mathbf{a}^+, \mathbf{r}}(z^{'*}_{K} \mid 
                             \mathbf{\overline{s}}^{'*}_{K},
                             \mathbf{\overline{a}}_{K-1}^+,
                             \mathbf{\overline{r}}_{K-1}, 
                             \mathbf{\overline{z}}^{'*}_{K-1})   \\
                 &  \underbrace{p_{\mathbf{a}^+, \mathbf{r}}}_{\ast}(s^{'*}_{K} \mid 
                             \mathbf{\overline{a}}_{K-1}^+
                             \mathbf{\overline{r}}_{K-1}, 
                             \mathbf{\overline{z}}^{'*}_{K-1},
                             \mathbf{\overline{s}}^{'*}_{K-1}) 
            \end{Bmatrix*}
\end{align*}

The equality follows simply by applying Lemma \ref{lemma49} (consistency). 

By Lemma \ref{lemma: indgenlemma} (Incomplete collision for non-ancestors), we have that the following independence holds

\begin{align*}
    \Big(\mathbb{A}_{K} (\mathbf{a^{\dagger}}, \mathbf{r}), \mathbb{R}_{K} (\mathbf{a^{\dagger}}, \mathbf{r})\Big)
        \CI 
            \mathbb{S}_{K}(\mathbf{a^{\dagger}}, \mathbf{r})
        \mid
            \overline{\mathbb{Z}}^{'*}_{K}(\mathbf{a^{\dagger}}, \mathbf{r}), 
            \overline{\mathbb{S}}^{'*}_{K-1}(\mathbf{a^{\dagger}}, \mathbf{r}),     
            \overline{\mathbb{A}}_{K-1}(\mathbf{a^{\dagger}}, \mathbf{r}),
            \overline{\mathbb{R}}_{K-1}(\mathbf{a^{\dagger}}, \mathbf{r}).
    \end{align*}

Then, by condition \eqref{eq: indgenlemma3}, exchangeability condition \eqref{eq: seqex} and laws of probability we start the following panel:

\begin{align*}
= & p_{\mathbf{a}^+, \mathbf{r}}(a_K, r_K \mid
                             \mathbf{\overline{z}}^{'*}_{K},
                             \mathbf{\overline{s}}^{'*}_{K-1},
                             \mathbf{\overline{a}}_{K-1}^+,
                             \mathbf{\overline{r}}_{K-1}) \\
       \sum\limits_{s^{'*}_{K}} &               
            \begin{Bmatrix*}[l]
                 &   p_{\mathbf{a}^+, \mathbf{r}}(y, z^{'*}_{K}, s^{'*}_{K} \mid 
                            \mathbf{\overline{a}}_{K-1}^+, 
                            \mathbf{\overline{r}}_{K-1}, 
                            \mathbf{\overline{z}}^{'*}_{K-1},
                            \mathbf{\overline{s}}^{'*}_{K-1}
                            )
            \end{Bmatrix*} \\
= & p_{\mathbf{a}^+, \mathbf{r}}(a_K, r_K \mid
                             \mathbf{\overline{z}}^{'*}_{K},
                             \mathbf{\overline{s}}^{'*}_{K-1},
                             \mathbf{\overline{a}}_{K-1}^+,
                             \mathbf{\overline{r}}_{K-1}) \\
                 &   p_{\mathbf{a}^+, \mathbf{r}}(\underbrace{y, z^{'*}_{K}}_{\ast} \mid 
                            \mathbf{\overline{a}}_{K-1}^+, 
                            \mathbf{\overline{r}}_{K-1}, 
                            \mathbf{\overline{z}}^{'*}_{K-1}, 
                            \mathbf{\overline{s}}^{'*}_{K-1}) \\
= & p_{\mathbf{a}^+, \mathbf{r}}(a_K, r_K \mid
                             \mathbf{\overline{z}}^{'*}_{K},
                             \mathbf{\overline{s}}^{'*}_{K-1},
                             \underbrace{\mathbf{\overline{a}}_{K-2}^+,
                             \mathbf{\overline{r}}_{K-2}}_{\ast\ast}) \\
                 &   p_{\mathbf{a}^+, \mathbf{r}}(y, z^{'*}_{K} \mid 
                            \underbrace{ \mathbf{\overline{a}}_{K-2}^+, 
                    \mathbf{\overline{r}}_{K-2}}_{\ast}, 
                            \mathbf{\overline{z}}^{'*}_{K-1}, 
                            \mathbf{\overline{s}}^{'*}_{K-1})
\end{align*}

The second equality follows by laws of probability and the third by conditions \eqref{eq: indgenlemma4} and \eqref{eq: indgenlemma5} of Lemma \ref{lemma: indgenlemma2} (Collision impossibility for outcome ancestors).

Thus we have:

\begin{align*}
& \begin{pmatrix*}[l] 
    \sum\limits_{s^{'*}_{1}} & 
         \begin{pmatrix*}[l] 
     &   p(a_{1}, r_{1} \mid
                     \mathbf{\overline{z}}^{'*}_{1},
                     \mathbf{\overline{s}}^{'*}_{1}) \\
         &   p(z^{'*}_{1} \mid 
                     s^{'*}_{1})   \\
         &  p(s^{'*}_{1} ) \\ 
        & \vdots \\
&    \cdots \begin{pmatrix*}[l] 
   \sum\limits_{s^{'*}_{K-2}} & 
         \begin{pmatrix*}[l] 
         &   p(a_{K-2}, r_{K-2} \mid
                     \mathbf{\overline{z}}^{'*}_{K-2},
                     \mathbf{\overline{s}}^{'*}_{K-2},
                     \mathbf{\overline{a}}_{K-3}^+,
                     \mathbf{\overline{r}}_{K-3}) \\
         &   p(z^{'*}_{K-2} \mid 
                     \mathbf{\overline{s}}^{'*}_{K-2},
                     \mathbf{\overline{a}}_{K-3}^+,
                     \mathbf{\overline{r}}_{j-1}, 
                     \mathbf{\overline{z}}^{'*}_{K-3})   \\
         &  p(s^{'*}_{K-2} \mid 
                     \mathbf{\overline{a}}_{K-3}^+,
                     \mathbf{\overline{r}}_{K-3}, 
                     \mathbf{\overline{z}}^{'*}_{j-1},
                     \mathbf{\overline{s}}^{'*}_{K-3} \\
   \sum\limits_{s^{'*}_{K-1}} & 
         \begin{pmatrix*}[l] 
         &   p(a_{K-1}, r_{K-1} \mid
                     \mathbf{\overline{z}}^{'*}_{K-1},
                     \mathbf{\overline{s}}^{'*}_{K-1},
                     \mathbf{\overline{a}}_{K-2}^+,
                     \mathbf{\overline{r}}_{K-2}) \\
         &   p(z^{'*}_{K-1} \mid 
                     \mathbf{\overline{s}}^{'*}_{K-1},
                     \mathbf{\overline{a}}_{K-2}^+,
                     \mathbf{\overline{r}}_{j-1}, 
                     \mathbf{\overline{z}}^{'*}_{K-2})   \\
         &  p(s^{'*}_{K-1} \mid 
                     \mathbf{\overline{a}}_{K-2}^+,
                     \mathbf{\overline{r}}_{K-2}, 
                     \mathbf{\overline{z}}^{'*}_{K-2},
                     \mathbf{\overline{s}}^{'*}_{K-2}) \\ 
                & p_{\mathbf{a}^+, \mathbf{r}}(a_K, r_K \mid
                             \mathbf{\overline{z}}^{'*}_{K},
                             \mathbf{\overline{s}}^{'*}_{K-1},
                             \mathbf{\overline{a}}_{K-2}^+,
                             \mathbf{\overline{r}}_{K-2}) \\
                 &   p_{\mathbf{a}^+, \mathbf{r}}(y, z^{'*}_{K} \mid 
                            \mathbf{\overline{a}}_{K-2}^+, 
                            \mathbf{\overline{r}}_{K-2}, 
                            \mathbf{\overline{z}}^{'*}_{K-1},
                            \mathbf{\overline{s}}^{'*}_{K-1})
        \end{pmatrix*}
\end{pmatrix*} 
\end{pmatrix*}
\end{pmatrix*}
\end{pmatrix*}.
\end{align*}

Consider time point $K-1$:

\begin{align*}
   \sum\limits_{s^{'*}_{K-1}} & 
         \begin{pmatrix*}[l] 
         &   p(a_{K-1}, r_{K-1} \mid
                     \mathbf{\overline{z}}^{'*}_{K-1},
                     \mathbf{\overline{s}}^{'*}_{K-1},
                     \mathbf{\overline{a}}_{K-2}^+,
                     \mathbf{\overline{r}}_{K-2}) \\
         &   p(z^{'*}_{K-1} \mid 
                     \mathbf{\overline{s}}^{'*}_{K-1},
                     \mathbf{\overline{a}}_{K-2}^+,
                     \mathbf{\overline{r}}_{K-2}, 
                     \mathbf{\overline{z}}^{'*}_{K-2})   \\
         &  p(s^{'*}_{K-1} \mid 
                     \mathbf{\overline{a}}_{K-2}^+,
                     \mathbf{\overline{r}}_{K-2}, 
                     \mathbf{\overline{z}}^{'*}_{K-2},
                     \mathbf{\overline{s}}^{'*}_{K-2}) \\ 
                & p_{\mathbf{a}^+, \mathbf{r}}(a_K, r_K \mid
                             \mathbf{\overline{z}}^{'*}_{K},
                             \mathbf{\overline{s}}^{'*}_{K-1},
                             \mathbf{\overline{a}}_{K-2}^+,
                             \mathbf{\overline{r}}_{K-2}) \\
                 &   p_{\mathbf{a}^+, \mathbf{r}}(y, z^{'*}_{K} \mid 
                            \mathbf{\overline{a}}_{K-2}^+, 
                            \mathbf{\overline{r}}_{K-2}, 
                            \mathbf{\overline{z}}^{'*}_{K-1},
                            \mathbf{\overline{s}}^{'*}_{K-1})
        \end{pmatrix*}\\
=       \sum\limits_{s^{'*}_{K-1}} & 
         \begin{pmatrix*}[l] 
         &   p_{\mathbf{a}^+, \mathbf{r}}(y \mid 
                    \mathbf{\overline{a}}_{K-2}^+, 
                    \mathbf{\overline{r}}_{K-2}, 
                    \mathbf{\overline{z}}^{'*}_{K},
                    \mathbf{\overline{s}}^{'*}_{K-1}) \\
        & p_{\mathbf{a}^+, \mathbf{r}}(a_K, r_K \mid
                     \mathbf{\overline{z}}^{'*}_{K},
                     \mathbf{\overline{s}}^{'*}_{K-1},
                     \mathbf{\overline{a}}_{K-2}^+,
                     \mathbf{\overline{r}}_{K-2}) \\
         &   p_{\mathbf{a}^+, \mathbf{r}}(z^{'*}_{K} \mid 
                    \mathbf{\overline{a}}_{K-2}^+, 
                    \mathbf{\overline{r}}_{K-2}, 
                    \mathbf{\overline{z}}^{'*}_{K-1},
                    \mathbf{\overline{s}}^{'*}_{K-1}) \\
         &   p_{\mathbf{a}^+, \mathbf{r}}(a_{K-1}, r_{K-1} \mid
                     \mathbf{\overline{z}}^{'*}_{K-1},
                     \mathbf{\overline{s}}^{'*}_{K-1},
                     \mathbf{\overline{a}}_{K-2}^+,
                     \mathbf{\overline{r}}_{K-2}) \\
         &   p_{\mathbf{a}^+, \mathbf{r}}(z^{'*}_{K-1} \mid 
                     \mathbf{\overline{s}}^{'*}_{K-1},
                     \mathbf{\overline{a}}_{K-2}^+,
                     \mathbf{\overline{r}}_{K-2}, 
                     \mathbf{\overline{z}}^{'*}_{K-2})   \\
         &  p_{\mathbf{a}^+, \mathbf{r}}(s^{'*}_{K-1} \mid 
                     \mathbf{\overline{a}}_{K-2}^+,
                     \mathbf{\overline{r}}_{K-2}, 
                     \mathbf{\overline{z}}^{'*}_{K-2},
                     \mathbf{\overline{s}}^{'*}_{K-2}) 
        \end{pmatrix*} 
\end{align*}

By Lemma \ref{lemma: indgenlemma} (Incomplete collision for non-ancestors), we have that the following independence holds

\begin{align*}
    \Big(\mathbb{A}_{K-1} (\mathbf{a^{\dagger}}, \mathbf{r}), \mathbb{R}_{K-1} (\mathbf{a^{\dagger}}, \mathbf{r}) \Big)
        \CI 
            \mathbb{S}_{K-1}(\mathbf{a^{\dagger}}, \mathbf{r})
        \mid
            \overline{\mathbb{Z}}^{'*}_{K-1}(\mathbf{a^{\dagger}}, \mathbf{r}), 
            \overline{\mathbb{S}}^{'*}_{K-2}(\mathbf{a^{\dagger}}, \mathbf{r}),     
            \overline{\mathbb{A}}_{K-2}(\mathbf{a^{\dagger}}, \mathbf{r}),
            \overline{\mathbb{R}}_{K-2}(\mathbf{a^{\dagger}}, \mathbf{r}), 
    \end{align*}

and that one of the two following independencies hold:

\begin{itemize}
    \item [$(K-1)(i)$] 
    \begin{align*}
    \Big(\mathbb{A}_{K} (\mathbf{a^{\dagger}}, \mathbf{r}), \mathbb{R}_{K} (\mathbf{a^{\dagger}}, \mathbf{r}) \Big)
        \CI 
            \mathbb{S}_{K-1}(\mathbf{a^{\dagger}}, \mathbf{r})
        \mid
            \overline{\mathbb{Z}}^{'*}_{K}(\mathbf{a^{\dagger}}, \mathbf{r}), 
            \overline{\mathbb{S}}^{'*}_{K-2}(\mathbf{a^{\dagger}}, \mathbf{r}),
            \overline{\mathbb{A}}_{K-2}(\mathbf{a^{\dagger}}, \mathbf{r}),
            \overline{\mathbb{R}}_{K-2}(\mathbf{a^{\dagger}}, \mathbf{r}), 
    \end{align*}
    \item [$(K-1)(ii)$] 
    \begin{align*}
        \mathbb{Y}(\mathbf{a^{\dagger}}, \mathbf{r})
         \CI 
            \mathbb{S}_{K-1}(\mathbf{a^{\dagger}}, \mathbf{r})
        \mid
            \overline{\mathbb{Z}}^{'*}_{K}(\mathbf{a^{\dagger}}, \mathbf{r}), 
            \overline{\mathbb{S}}^{'*}_{K-2}(\mathbf{a^{\dagger}}, \mathbf{r}),
            \overline{\mathbb{A}}_{K-2}(\mathbf{a^{\dagger}}, \mathbf{r}),
            \overline{\mathbb{r}}_{K-2}(\mathbf{a^{\dagger}}, \mathbf{r}),
    \end{align*}
\end{itemize}

Under $(K-1)(i)$ we have:

\begin{align*}
=    &   p_{\mathbf{a}^+, \mathbf{r}}(a_{K-1}, r_{K-1} \mid
                     \mathbf{\overline{z}}^{'*}_{K-1},
                     \mathbf{\overline{s}}^{'*}_{K-2},
                     \mathbf{\overline{a}}_{K-2}^+,
                     \mathbf{\overline{r}}_{K-2}) \\
        & p_{\mathbf{a}^+, \mathbf{r}}(a_{K}, r_K \mid
                     \mathbf{\overline{z}}^{'*}_{K},
                     \mathbf{\overline{s}}^{'*}_{K-2},
                     \mathbf{\overline{a}}_{K-2}^+,
                     \mathbf{\overline{r}}_{K-2}) \\
        \sum\limits_{s^{'*}_{K-1}} & 
         \begin{pmatrix*}[l] 
         &   p_{\mathbf{a}^+, \mathbf{r}}(y \mid 
                    \mathbf{\overline{a}}_{K-2}^+, 
                    \mathbf{\overline{r}}_{K-2}, 
                    \mathbf{\overline{z}}^{'*}_{K},
                    \mathbf{\overline{s}}^{'*}_{K-1}) \\
         &   p_{\mathbf{a}^+, \mathbf{r}}(z^{'*}_{K} \mid 
                    \mathbf{\overline{a}}_{K-2}^+, 
                    \mathbf{\overline{r}}_{K-2}, 
                    \mathbf{\overline{z}}^{'*}_{K-1},
                    \mathbf{\overline{s}}^{'*}_{K-1}) \\
         &   p_{\mathbf{a}^+, \mathbf{r}}(z^{'*}_{K-1} \mid 
                     \mathbf{\overline{s}}^{'*}_{K-1},
                     \mathbf{\overline{a}}_{K-2}^+,
                     \mathbf{\overline{r}}_{K-2}, 
                     \mathbf{\overline{z}}^{'*}_{K-2})   \\
         &  p_{\mathbf{a}^+, \mathbf{r}}(s^{'*}_{K-1} \mid 
                     \mathbf{\overline{a}}_{K-2}^+,
                     \mathbf{\overline{r}}_{K-2}, 
                     \mathbf{\overline{z}}^{'*}_{K-2},
                     \mathbf{\overline{s}}^{'*}_{K-2}) 
        \end{pmatrix*} \\ 
=    &   p_{\mathbf{a}^+, \mathbf{r}}(a_{K-1}, r_{K-1} \mid
                     \mathbf{\overline{z}}^{'*}_{K-1},
                     \mathbf{\overline{s}}^{'*}_{K-2},
                     \mathbf{\overline{a}}_{K-2}^+,
                     \mathbf{\overline{r}}_{K-2}) \\
        & p_{\mathbf{a}^+, \mathbf{r}}(a_{K}, r_K \mid
                     \mathbf{\overline{z}}^{'*}_{K},
                     \mathbf{\overline{s}}^{'*}_{K-2},
                     \mathbf{\overline{a}}_{K-2}^+,
                     \mathbf{\overline{r}}_{K-2}) \\
        \sum\limits_{s^{'*}_{K-1}} & 
         \begin{pmatrix*}[l] 
         &   p_{\mathbf{a}^+, \mathbf{r}}(y, \underline{\mathbf{z}}^{'*}_{K-1}, s^{'*}_{K-1} \mid 
                     \mathbf{\overline{a}}_{K-2}^+,
                     \mathbf{\overline{r}}_{K-2}, 
                     \mathbf{\overline{z}}^{'*}_{K-2},
                     \mathbf{\overline{s}}^{'*}_{K-2}) 
        \end{pmatrix*} \\ 
=    &   p_{\mathbf{a}^+, \mathbf{r}}(a_{K-1}, r_{K-1} \mid
                     \mathbf{\overline{z}}^{'*}_{K-1},
                     \mathbf{\overline{s}}^{'*}_{K-2},
                     \mathbf{\overline{a}}_{K-2}^+,
                     \mathbf{\overline{r}}_{K-2}) \\
        & p_{\mathbf{a}^+, \mathbf{r}}(a_{K}, r_K \mid
                     \mathbf{\overline{z}}^{'*}_{K},
                     \mathbf{\overline{s}}^{'*}_{K-2},
                     \mathbf{\overline{a}}_{K-2}^+,
                     \mathbf{\overline{r}}_{K-2}) \\
         &   p_{\mathbf{a}^+, \mathbf{r}}(y, \underline{\mathbf{z}}^{'*}_{K-1} \mid 
                     \mathbf{\overline{a}}_{K-2}^+,
                     \mathbf{\overline{r}}_{K-2}, 
                     \mathbf{\overline{z}}^{'*}_{K-2},
                     \mathbf{\overline{s}}^{'*}_{K-2})  \\ 
=    &   p_{\mathbf{a}^+, \mathbf{r}}(a_{K-1}, r_{K-1} \mid
                     \mathbf{\overline{z}}^{'*}_{K-1},
                     \mathbf{\overline{s}}^{'*}_{K-2},
                     \underbrace{\mathbf{\overline{a}}_{K-3}^+,
                 \mathbf{\overline{r}}_{K-3}}_{\ast\ast}) \\
        & p_{\mathbf{a}^+, \mathbf{r}}(a_{K}, r_K \mid
                     \mathbf{\overline{z}}^{'*}_{K},
                     \mathbf{\overline{s}}^{'*}_{K-2},
                    \underbrace{ \mathbf{\overline{a}}_{K-3}^+,
                 \mathbf{\overline{r}}_{K-3}}_{\ast\ast}) \\
         &   p_{\mathbf{a}^+, \mathbf{r}}(y, \underline{\mathbf{z}}^{'*}_{K-1} \mid 
                     \underbrace{\mathbf{\overline{a}}_{K-3}^+,
                     \mathbf{\overline{r}}_{K-3}}_{\ast}, 
                     \mathbf{\overline{z}}^{'*}_{K-2},
                     \mathbf{\overline{s}}^{'*}_{K-2})  \\ 
\end{align*}

The first equality follows immediately from the independence in $(K-1)(i)$. The second and third equalities follows by laws of probability. The fourth follows by conditions \eqref{eq: indgenlemma4} and \eqref{eq: indgenlemma5} of Lemma \ref{lemma: indgenlemma2} (Collision impossibility for outcome ancestors).

Under $(K-1)(ii)$ we have: 

\begin{align*}
=    &   p_{\mathbf{a}^+, \mathbf{r}}(a_{K-1}, r_{K-1} \mid
                     \mathbf{\overline{z}}^{'*}_{K-1},
                     \mathbf{\overline{s}}^{'*}_{K-2},
                     \mathbf{\overline{a}}_{K-2}^+,
                     \mathbf{\overline{r}}_{K-2}) \\
         &   p_{\mathbf{a}^+, \mathbf{r}}(y \mid 
                    \mathbf{\overline{a}}_{K-2}^+, 
                    \mathbf{\overline{r}}_{K-2}, 
                    \mathbf{\overline{z}}^{'*}_{K}, 
                    \mathbf{\overline{s}}^{'*}_{K-2}) \\
        \sum\limits_{s^{'*}_{K-1}} & 
         \begin{pmatrix*}[l] 
        & p_{\mathbf{a}^+, \mathbf{r}}(a_{K}, r_K \mid
                     \mathbf{\overline{z}}^{'*}_{K},
                     \mathbf{\overline{s}}^{'*}_{K-1},
                     \mathbf{\overline{a}}_{K-2}^+,
                     \mathbf{\overline{r}}_{K-2}) \\
         &   p_{\mathbf{a}^+, \mathbf{r}}(z^{'*}_{K} \mid 
                    \mathbf{\overline{a}}_{K-2}^+, 
                    \mathbf{\overline{r}}_{K-2}, 
                    \mathbf{\overline{z}}^{'*}_{K-1}, 
                    \mathbf{\overline{s}}^{'*}_{K-1}) \\
         &   p_{\mathbf{a}^+, \mathbf{r}}(z^{'*}_{K-1} \mid 
                     \mathbf{\overline{s}}^{'*}_{K-1},
                     \mathbf{\overline{a}}_{K-2}^+,
                     \mathbf{\overline{r}}_{K-2}, 
                     \mathbf{\overline{z}}^{'*}_{K-2})   \\
         &  p_{\mathbf{a}^+, \mathbf{r}}(s^{'*}_{K-1} \mid 
                     \mathbf{\overline{a}}_{K-2}^+,
                     \mathbf{\overline{r}}_{K-2}, 
                     \mathbf{\overline{z}}^{'*}_{K-2},
                     \mathbf{\overline{s}}^{'*}_{K-2}) 
        \end{pmatrix*} \\ 
=    &   p_{\mathbf{a}^+, \mathbf{r}}(a_{K-1}, r_{K-1} \mid
                     \mathbf{\overline{z}}^{'*}_{K-1},
                     \mathbf{\overline{s}}^{'*}_{K-2},
                     \mathbf{\overline{a}}_{K-2}^+,
                     \mathbf{\overline{r}}_{K-2}) \\
         &   p_{\mathbf{a}^+, \mathbf{r}}(y \mid 
                    \mathbf{\overline{a}}_{K-2}^+, 
                    \mathbf{\overline{r}}_{K-2}, 
                    \mathbf{\overline{z}}^{'*}_{K}, 
                    \mathbf{\overline{s}}^{'*}_{K-2}) \\
        \sum\limits_{s^{'*}_{K-1}} & 
         \begin{pmatrix*}[l] 
         &   p_{\mathbf{a}^+, \mathbf{r}}(a_{K}, r_K, \underline{\mathbf{z}}^{'*}_{K-1}, s^{'*}_{K-1} \mid 
                     \mathbf{\overline{a}}_{K-2}^+,
                     \mathbf{\overline{r}}_{K-2}, 
                     \mathbf{\overline{z}}^{'*}_{K-2},
                     \mathbf{\overline{s}}^{'*}_{K-2}) 
        \end{pmatrix*} \\ 
=    &   p_{\mathbf{a}^+, \mathbf{r}}(a_{K-1}, r_{K-1} \mid
                     \mathbf{\overline{z}}^{'*}_{K-1},
                     \mathbf{\overline{s}}^{'*}_{K-2},
                     \underbrace{\mathbf{\overline{a}}_{K-3}^+,
                     \mathbf{\overline{r}}_{K-3}}_{\ast,\ast}) \\
         &   p_{\mathbf{a}^+, \mathbf{r}}(y \mid 
                   \underbrace{ \mathbf{\overline{a}}_{K-3}^+, 
                    \mathbf{\overline{r}}_{K-3}}_{\ast,\ast}, 
                    \mathbf{\overline{z}}^{'*}_{K}, 
                    \mathbf{\overline{s}}^{'*}_{K-2}) \\
         &   p_{\mathbf{a}^+, \mathbf{r}}(a_{K}, r_K, \underline{\mathbf{z}}^{'*}_{K-1}\mid 
                     \underbrace{\mathbf{\overline{a}}_{K-3}^+,
                     \mathbf{\overline{r}}_{K-3}}_{\ast}, 
                     \mathbf{\overline{z}}^{'*}_{K-2},
                     \mathbf{\overline{s}}^{'*}_{K-2})  \\ 
=    &   p_{\mathbf{a}^+, \mathbf{r}}(a_{K-1}, r_{K-1} \mid
                     \mathbf{\overline{z}}^{'*}_{K-1},
                     \mathbf{\overline{s}}^{'*}_{K-2},
                     \mathbf{\overline{a}}_{K-3}^+,
                     \mathbf{\overline{r}}_{K-3}) \\
        & p_{\mathbf{a}^+, \mathbf{r}}(a_{K}, r_K \mid
                     \mathbf{\overline{z}}^{'*}_{K},
                     \mathbf{\overline{s}}^{'*}_{K-2},
                     \mathbf{\overline{a}}_{K-3}^+,
                     \mathbf{\overline{r}}_{K-3}) \\
         &   p_{\mathbf{a}^+, \mathbf{r}}(y, \underline{\mathbf{z}}^{'*}_{K-1} \mid 
                     \mathbf{\overline{a}}_{K-3}^+,
                     \mathbf{\overline{r}}_{K-3}, 
                     \mathbf{\overline{z}}^{'*}_{K-2},
                     \mathbf{\overline{s}}^{'*}_{K-2})  \\ 
\end{align*}

The first equality follows immediately from the independence in $(K-1)(ii)$. The second equality follows by laws of probability. The third follows by laws of probability, conditions \eqref{eq: indgenlemma4} and \eqref{eq: indgenlemma5} of Lemma \ref{lemma: indgenlemma2} (Collision impossibility for outcome ancestors). The fourth re-arranges terms.

Thus under either $(K-1)(i)$ or $(K-1)(ii)$ we have:

\begin{align*}
    \sum\limits_{s^{'*}_{1}} & 
         \begin{pmatrix*}[l] 
     &   p(a_{1}, r_{1} \mid
                     \mathbf{\overline{z}}^{'*}_{1},
                     \mathbf{\overline{s}}^{'*}_{1}) \\
         &   p(z^{'*}_{1} \mid 
                     s^{'*}_{1})   \\
         &  p(s^{'*}_{1} ) \\ 
        & \vdots \\
&    \cdots \begin{pmatrix*}[l] 
   \sum\limits_{s^{'*}_{K-2}} & 
         \begin{pmatrix*}[l] 
         &   p(a_{K-2}, r_{K-2} \mid
                     \mathbf{\overline{z}}^{'*}_{K-2},
                     \mathbf{\overline{s}}^{'*}_{K-2},
                     \mathbf{\overline{a}}_{K-3}^+,
                     \mathbf{\overline{r}}_{K-3}) \\
         &   p(z^{'*}_{K-2} \mid 
                     \mathbf{\overline{s}}^{'*}_{K-2},
                     \mathbf{\overline{a}}_{K-3}^+,
                     \mathbf{\overline{r}}_{K-3}, 
                     \mathbf{\overline{z}}^{'*}_{K-3})   \\
         &  p(s^{'*}_{K-2} \mid 
                     \mathbf{\overline{a}}_{K-3}^+,
                     \mathbf{\overline{r}}_{K-3}, 
                     \mathbf{\overline{z}}^{'*}_{K-3},
                     \mathbf{\overline{s}}^{'*}_{K-3} \\
&   p_{\mathbf{a}^+, \mathbf{r}}(a_{K-1}, r_{K-1} \mid
                     \mathbf{\overline{z}}^{'*}_{K-1},
                     \mathbf{\overline{s}}^{'*}_{K-2},
                     \mathbf{\overline{a}}_{K-3}^+,
                     \mathbf{\overline{r}}_{K-3}) \\
        & p_{\mathbf{a}^+, \mathbf{r}}(a_{K}, r_K \mid
                     \mathbf{\overline{z}}^{'*}_{K},
                     \mathbf{\overline{s}}^{'*}_{K-2},
                     \mathbf{\overline{a}}_{K-3}^+,
                     \mathbf{\overline{r}}_{K-3}) \\
         &   p_{\mathbf{a}^+, \mathbf{r}}(y, \underline{\mathbf{z}}^{'*}_{K-1} \mid 
                     \mathbf{\overline{a}}_{K-3}^+,
                     \mathbf{\overline{r}}_{K-3}, 
                     \mathbf{\overline{z}}^{'*}_{K-2},
                     \mathbf{\overline{s}}^{'*}_{K-2}) 
\end{pmatrix*} 
\end{pmatrix*}
\end{pmatrix*}.
\end{align*}

Consider time point $K-2$:

\begin{align*}
& \sum\limits_{s^{'*}_{K-2}}  
         \begin{pmatrix*}[l] 
         &   p(a_{K-2}, r_{K-2} \mid
                     \mathbf{\overline{z}}^{'*}_{K-2},
                     \mathbf{\overline{s}}^{'*}_{K-2},
                     \mathbf{\overline{a}}_{K-3}^+,
                     \mathbf{\overline{r}}_{K-3}) \\
         &   p(z^{'*}_{K-2} \mid 
                     \mathbf{\overline{s}}^{'*}_{K-2},
                     \mathbf{\overline{a}}_{K-3}^+,
                     \mathbf{\overline{r}}_{K-3}, 
                     \mathbf{\overline{z}}^{'*}_{K-3})   \\
         &  p(s^{'*}_{K-2} \mid 
                     \mathbf{\overline{a}}_{K-3}^+,
                     \mathbf{\overline{r}}_{K-3}, 
                     \mathbf{\overline{z}}^{'*}_{K-3},
                     \mathbf{\overline{s}}^{'*}_{K-3} \\
&   p_{\mathbf{a}^+, \mathbf{r}}(a_{K-1}, r_{K-1} \mid
                     \mathbf{\overline{z}}^{'*}_{K-1},
                     \mathbf{\overline{s}}^{'*}_{K-2},
                     \mathbf{\overline{a}}_{K-3}^+,
                     \mathbf{\overline{r}}_{K-3}) \\
        & p_{\mathbf{a}^+, \mathbf{r}}(a_{K}, r_K \mid
                     \mathbf{\overline{z}}^{'*}_{K},
                     \mathbf{\overline{s}}^{'*}_{K-2},
                     \mathbf{\overline{a}}_{K-3}^+,
                     \mathbf{\overline{r}}_{K-3}) \\
         &   p_{\mathbf{a}^+, \mathbf{r}}(y, \underline{\mathbf{z}}^{'*}_{K-1} \mid 
                     \mathbf{\overline{a}}_{K-3}^+,
                     \mathbf{\overline{r}}_{K-3}, 
                     \mathbf{\overline{z}}^{'*}_{K-2},
                     \mathbf{\overline{s}}^{'*}_{K-2}) 
\end{pmatrix*} \\
= & \sum\limits_{s^{'*}_{K-2}}  
         \begin{pmatrix*}[l] 
        &   p_{\mathbf{a}^+, \mathbf{r}}(y \mid 
                     \mathbf{\overline{a}}_{K-3}^+,
                     \mathbf{\overline{r}}_{K-3}, 
                     \mathbf{\overline{z}}^{'*}_{K},
                     \mathbf{\overline{s}}^{'*}_{K-2}) \\
        & p_{\mathbf{a}^+, \mathbf{r}}(a_{K}, r_K \mid
                     \mathbf{\overline{z}}^{'*}_{K},
                     \mathbf{\overline{s}}^{'*}_{K-2},
                     \mathbf{\overline{a}}_{K-3}^+,
                     \mathbf{\overline{r}}_{K-3}) \\
        &   p_{\mathbf{a}^+, \mathbf{r}}(z^{'*}_{K} \mid 
                     \mathbf{\overline{a}}_{K-3}^+,
                     \mathbf{\overline{r}}_{K-3}, 
                     \mathbf{\overline{z}}^{'*}_{K-1},
                     \mathbf{\overline{s}}^{'*}_{K-2}) \\
        &   p_{\mathbf{a}^+, \mathbf{r}}(a_{K-1}, r_{K-1} \mid
                     \mathbf{\overline{z}}^{'*}_{K-1},
                     \mathbf{\overline{s}}^{'*}_{K-2},
                     \mathbf{\overline{a}}_{K-2}^+,
                     \mathbf{\overline{r}}_{K-3}) \\
        &   p_{\mathbf{a}^+, \mathbf{r}}(z^{'*}_{K-1} \mid 
                     \mathbf{\overline{a}}_{K-3}^+,
                     \mathbf{\overline{r}}_{K-3}, 
                     \mathbf{\overline{z}}^{'*}_{K-2},
                     \mathbf{\overline{s}}^{'*}_{K-2}) \\
         &   p_{\mathbf{a}^+, \mathbf{r}}(a_{K-2}, r_{K-2} \mid
                     \mathbf{\overline{z}}^{'*}_{K-2},
                     \mathbf{\overline{s}}^{'*}_{K-2},
                     \mathbf{\overline{a}}_{K-3}^+,
                     \mathbf{\overline{r}}_{K-3}) \\
         &   p_{\mathbf{a}^+, \mathbf{r}}(z^{'*}_{K-2} \mid 
                     \mathbf{\overline{s}}^{'*}_{K-2},
                     \mathbf{\overline{a}}_{K-3}^+,
                     \mathbf{\overline{r}}_{K-3}, 
                     \mathbf{\overline{z}}^{'*}_{K-3})   \\
         &  p_{\mathbf{a}^+, \mathbf{r}}(s^{'*}_{K-2} \mid 
                     \mathbf{\overline{a}}_{K-3}^+,
                     \mathbf{\overline{r}}_{K-3}, 
                     \mathbf{\overline{z}}^{'*}_{K-3},
                     \mathbf{\overline{s}}^{'*}_{K-3}) \\
\end{pmatrix*} \\
\end{align*}

By Lemma \ref{lemma: indgenlemma}, we have that the following independence holds:

\begin{align*}
    \Big(\mathbb{A}_{K-2} (\mathbf{a^{\dagger}}, \mathbf{r}), \mathbb{R}_{K-2} (\mathbf{a^{\dagger}}, \mathbf{r})\Big)
        \CI 
            \mathbb{S}_{K-2}(\mathbf{a^{\dagger}}, \mathbf{r})
        \mid
            \overline{\mathbb{Z}}^{'*}_{K-2}(\mathbf{a^{\dagger}}, \mathbf{r}), 
            \overline{\mathbb{S}}^{'*}_{K-3}(\mathbf{a^{\dagger}}, \mathbf{r})
            \overline{\mathbb{A}}_{K-3}(\mathbf{a^{\dagger}}, \mathbf{r}),
            \overline{\mathbb{R}}_{K-3}(\mathbf{a^{\dagger}}, \mathbf{r}), 
    \end{align*}

and that one of the three following independencies hold:

\begin{itemize}
    \item [$(K-2)(i)$] 
    \begin{align*}
          \Big(\mathbb{A}_K (\mathbf{a^{\dagger}}, \mathbf{r}), \mathbb{R}_K (\mathbf{a^{\dagger}}, \mathbf{r})\Big)
        \CI &
            \mathbb{S}_{K-2}(\mathbf{a^{\dagger}}, \mathbf{r})
        \mid
            \overline{\mathbb{Z}}^{'*}_{K}(\mathbf{a^{\dagger}}, \mathbf{r}), 
            \overline{\mathbb{S}}^{'*}_{K-3}(\mathbf{a^{\dagger}}, \mathbf{r}),
            \overline{\mathbb{A}}_{K-3}(\mathbf{a^{\dagger}}, \mathbf{r}),
            \overline{\mathbb{R}}_{K-3}(\mathbf{a^{\dagger}}, \mathbf{r}), \text{ and } \\
        \Big(\mathbb{A}_{K-1}(\mathbf{a^{\dagger}}, \mathbf{r}),    \mathbb{R}_{K-1} (\mathbf{a^{\dagger}}, \mathbf{r})\Big)
        \CI &
            \mathbb{S}_{K-2}(\mathbf{a^{\dagger}}, \mathbf{r})
        \mid
            \overline{\mathbb{Z}}^{'*}_{K-1}(\mathbf{a^{\dagger}}, \mathbf{r}), 
            \overline{\mathbb{S}}^{'*}_{K-3}(\mathbf{a^{\dagger}}, \mathbf{r}),
            \overline{\mathbb{A}}_{K-3}(\mathbf{a^{\dagger}}, \mathbf{r}),
            \overline{\mathbb{R}}_{K-3}(\mathbf{a^{\dagger}}, \mathbf{r})
    \end{align*}
    \item [$(K-2)(ii)$] 
        \begin{align*}
          \mathbb{Y} (\mathbf{a^{\dagger}}, \mathbf{r})
        \CI &
            \mathbb{S}_{K-2}(\mathbf{a^{\dagger}}, \mathbf{r})
        \mid
            \overline{\mathbb{Z}}^{'*}_{K}(\mathbf{a^{\dagger}}, \mathbf{r}), 
            \overline{\mathbb{S}}^{'*}_{K-3}(\mathbf{a^{\dagger}}, \mathbf{r}),
            \overline{\mathbb{A}}_{K-3}(\mathbf{a^{\dagger}}, \mathbf{r}),
            \overline{\mathbb{R}}_{K-3}(\mathbf{a^{\dagger}}, \mathbf{r}), \text{ and } \\
          \Big(\mathbb{A}_{K-1} (\mathbf{a^{\dagger}}, \mathbf{r}), \mathbb{R}_{K-1} (\mathbf{a^{\dagger}}, \mathbf{r})\Big)
        \CI &
            \mathbb{S}_{K-2}(\mathbf{a^{\dagger}}, \mathbf{r})
        \mid
            \overline{\mathbb{Z}}^{'*}_{K-1}(\mathbf{a^{\dagger}}, \mathbf{r}), 
            \overline{\mathbb{S}}^{'*}_{K-3}(\mathbf{a^{\dagger}}, \mathbf{r}),
            \overline{\mathbb{A}}_{K-3}(\mathbf{a^{\dagger}}, \mathbf{r}),
            \overline{\mathbb{R}}_{K-3}(\mathbf{a^{\dagger}}, \mathbf{r})
    \end{align*}
    \item [$(K-2)(iii)$] 
        \begin{align*}
    \mathbb{Y} (\mathbf{a^{\dagger}}, \mathbf{r})
        \CI &
            \mathbb{S}_{K-2}(\mathbf{a^{\dagger}}, \mathbf{r})
        \mid
            \overline{\mathbb{Z}}^{'*}_{K}(\mathbf{a^{\dagger}}, \mathbf{r}), 
            \overline{\mathbb{S}}^{'*}_{K-3}(\mathbf{a^{\dagger}}, \mathbf{r}),
            \overline{\mathbb{A}}_{K-3}(\mathbf{a^{\dagger}}, \mathbf{r}),
            \overline{\mathbb{R}}_{K-3}(\mathbf{a^{\dagger}}, \mathbf{r}), \text{ and } \\
   \Big( \mathbb{A}_{K} (\mathbf{a^{\dagger}}, \mathbf{r}), \mathbb{R}_K (\mathbf{a^{\dagger}}, \mathbf{r})\Big)
        \CI &
            \mathbb{S}_{K-2}(\mathbf{a^{\dagger}}, \mathbf{r})
        \mid
            \overline{\mathbb{Z}}^{'*}_{K}(\mathbf{a^{\dagger}}, \mathbf{r}), 
            \overline{\mathbb{S}}^{'*}_{K-3}(\mathbf{a^{\dagger}}, \mathbf{r}),
            \overline{\mathbb{A}}_{K-3}(\mathbf{a^{\dagger}}, \mathbf{r}),
            \overline{\mathbb{R}}_{K-3}(\mathbf{a^{\dagger}}, \mathbf{r}), \text{ and } \\
    \mathbb{Z}^{'*}_K (\mathbf{a^{\dagger}}, \mathbf{r})
        \CI &
            \mathbb{S}_{K-2}(\mathbf{a^{\dagger}}, \mathbf{r})
        \mid
            \overline{\mathbb{Z}}^{'*}_{K-1}(\mathbf{a^{\dagger}}, \mathbf{r}), 
            \overline{\mathbb{S}}^{'*}_{K-3}(\mathbf{a^{\dagger}}, \mathbf{r}),
            \overline{\mathbb{A}}_{K-3}(\mathbf{a^{\dagger}}, \mathbf{r}),
            \overline{\mathbb{R}}_{K-3}(\mathbf{a^{\dagger}}, \mathbf{r}). 
    \end{align*}
\end{itemize}

Under $(K-2)(i)$ we have:

\begin{align*}
=         & p_{\mathbf{a}^+, \mathbf{r}}(a_{K}, r_K \mid
                     \mathbf{\overline{z}}^{'*}_{K},
                     \mathbf{\overline{s}}^{'*}_{K-3},
                     \mathbf{\overline{a}}_{K-3}^+,
                     \mathbf{\overline{r}}_{K-3}) \\
        &   p_{\mathbf{a}^+, \mathbf{r}}(a_{K-1}, r_{K-1} \mid
                     \mathbf{\overline{z}}^{'*}_{K-1},
                     \mathbf{\overline{s}}^{'*}_{K-3},
                     \mathbf{\overline{a}}_{K-3}^+,
                     \mathbf{\overline{r}}_{K-3}) \\            
        &   p_{\mathbf{a}^+, \mathbf{r}}(a_{K-2}, r_{K-2} \mid
                     \mathbf{\overline{z}}^{'*}_{K-2},
                     \mathbf{\overline{s}}^{'*}_{K-3},
                     \mathbf{\overline{a}}_{K-3}^+,
                     \mathbf{\overline{r}}_{K-3}) \\ 
& \sum\limits_{s^{'*}_{K-2}}  
         \begin{pmatrix*}[l] 
        &   p_{\mathbf{a}^+, \mathbf{r}}(y \mid 
                     \mathbf{\overline{a}}_{K-3}^+,
                     \mathbf{\overline{r}}_{K-3}, 
                     \mathbf{\overline{z}}^{'*}_{K},
                     \mathbf{\overline{s}}^{'*}_{K-2}) \\
        &   p_{\mathbf{a}^+, \mathbf{r}}(z^{'*}_{K} \mid 
                     \mathbf{\overline{a}}_{K-3}^+,
                     \mathbf{\overline{r}}_{K-3}, 
                     \mathbf{\overline{z}}^{'*}_{K-1},
                     \mathbf{\overline{s}}^{'*}_{K-2}) \\
        &   p_{\mathbf{a}^+, \mathbf{r}}(z^{'*}_{K-1} \mid 
                     \mathbf{\overline{a}}_{K-3}^+,
                     \mathbf{\overline{r}}_{K-3}, 
                     \mathbf{\overline{z}}^{'*}_{K-2},
                     \mathbf{\overline{s}}^{'*}_{K-2}) \\
         &   p_{\mathbf{a}^+, \mathbf{r}}(z^{'*}_{K-2} \mid 
                     \mathbf{\overline{s}}^{'*}_{K-2},
                     \mathbf{\overline{a}}_{K-3}^+,
                     \mathbf{\overline{r}}_{K-3}, 
                     \mathbf{\overline{z}}^{'*}_{K-3})   \\
         &  p_{\mathbf{a}^+, \mathbf{r}}(s^{'*}_{K-2} \mid 
                     \mathbf{\overline{a}}_{K-3}^+,
                     \mathbf{\overline{r}}_{K-3}, 
                     \mathbf{\overline{z}}^{'*}_{K-3K-3},
                     \mathbf{\overline{s}}^{'*}_{K-3}) \\
\end{pmatrix*} \\
=         & p_{\mathbf{a}^+, \mathbf{r}}(a_{K}, r_K \mid
                     \mathbf{\overline{z}}^{'*}_{K},
                     \mathbf{\overline{s}}^{'*}_{K-3},
                     \mathbf{\overline{a}}_{K-3}^+,
                     \mathbf{\overline{r}}_{K-3}) \\
        &   p_{\mathbf{a}^+, \mathbf{r}}(a_{K-1}, r_{K-1} \mid
                     \mathbf{\overline{z}}^{'*}_{K-1},
                     \mathbf{\overline{s}}^{'*}_{K-3},
                     \mathbf{\overline{a}}_{K-3}^+,
                     \mathbf{\overline{r}}_{K-3}) \\            
        &   p_{\mathbf{a}^+, \mathbf{r}}(a_{K-2}, r_{K-2} \mid
                     \mathbf{\overline{z}}^{'*}_{K-2},
                     \mathbf{\overline{s}}^{'*}_{K-3},
                     \mathbf{\overline{a}}_{K-3}^+,
                     \mathbf{\overline{r}}_{K-3}) \\ 
& \sum\limits_{s^{'*}_{K-2}}  
         \begin{pmatrix*}[l] 
        &   p_{\mathbf{a}^+, \mathbf{r}}(y, \underline{\mathbf{z}}^{'*}_{K-2} ,s^{'*}_{K-2} \mid 
                     \mathbf{\overline{a}}_{K-3}^+,
                     \mathbf{\overline{r}}_{K-3}, 
                     \mathbf{\overline{z}}^{'*}_{K-3},
                     \mathbf{\overline{s}}^{'*}_{K-3}) \\
\end{pmatrix*} \\
=         & p_{\mathbf{a}^+, \mathbf{r}}(a_{K}, r_K \mid
                     \mathbf{\overline{z}}^{'*}_{K},
                     \mathbf{\overline{s}}^{'*}_{K-3},
                     \mathbf{\overline{a}}_{K-4}^+,
                     \mathbf{\overline{r}}_{K-4}) \\
        &   p_{\mathbf{a}^+, \mathbf{r}}(a_{K-1}, r_{K-1} \mid
                     \mathbf{\overline{z}}^{'*}_{K-1},
                     \mathbf{\overline{s}}^{'*}_{K-3},
                     \mathbf{\overline{a}}_{K-4}^+,
                     \mathbf{\overline{r}}_{K-4}) \\            
        &   p_{\mathbf{a}^+, \mathbf{r}}(a_{K-2}, r_{K-2} \mid
                     \mathbf{\overline{z}}^{'*}_{K-2},
                     \mathbf{\overline{s}}^{'*}_{K-3},
                     \mathbf{\overline{a}}_{K-4}^+,
                     \mathbf{\overline{r}}_{K-4}) \\ 
        &   p_{\mathbf{a}^+, \mathbf{r}}(y, \underline{\mathbf{z}}^{'*}_{K-2}  \mid 
                     \mathbf{\overline{a}}_{K-4}^+,
                     \mathbf{\overline{r}}_{K-4}, 
                     \mathbf{\overline{z}}^{'*}_{K-3},
                     \mathbf{\overline{s}}^{'*}_{K-3}) \\
\end{align*}

Under $(K-2)(ii)$ we have:

\begin{align*}
=         & p_{\mathbf{a}^+, \mathbf{r}}(y \mid
                     \mathbf{\overline{z}}^{'*}_{K},
                     \mathbf{\overline{s}}^{'*}_{K-3},
                     \mathbf{\overline{a}}_{K-3}^+,
                     \mathbf{\overline{r}}_{K-3}) \\
        &   p_{\mathbf{a}^+, \mathbf{r}}(a_{K-1}, r_{K-1} \mid
                     \mathbf{\overline{z}}^{'*}_{K-1},
                     \mathbf{\overline{s}}^{'*}_{K-3},
                     \mathbf{\overline{a}}_{K-3}^+,
                     \mathbf{\overline{r}}_{K-3}) \\            
        &   p_{\mathbf{a}^+, \mathbf{r}}(a_{K-2}, r_{K-2} \mid
                     \mathbf{\overline{z}}^{'*}_{K-2},
                     \mathbf{\overline{s}}^{'*}_{K-3},
                     \mathbf{\overline{a}}_{K-3}^+,
                     \mathbf{\overline{r}}_{K-3}) \\ 
& \sum\limits_{s^{'*}_{K-2}}  
         \begin{pmatrix*}[l] 
        &   p_{\mathbf{a}^+, \mathbf{r}}(a_{K}, r_K \mid 
                     \mathbf{\overline{a}}_{K-3}^+,
                     \mathbf{\overline{r}}_{K-3}, 
                     \mathbf{\overline{z}}^{'*}_{K},
                     \mathbf{\overline{s}}^{'*}_{K-2}) \\
        &   p_{\mathbf{a}^+, \mathbf{r}}(z^{'*}_{K} \mid 
                     \mathbf{\overline{a}}_{K-3}^+,
                     \mathbf{\overline{r}}_{K-3}, 
                     \mathbf{\overline{z}}^{'*}_{K-1},
                     \mathbf{\overline{s}}^{'*}_{K-2}) \\
        &   p_{\mathbf{a}^+, \mathbf{r}}(z^{'*}_{K-1} \mid 
                     \mathbf{\overline{a}}_{K-3}^+,
                     \mathbf{\overline{r}}_{K-3}, 
                     \mathbf{\overline{z}}^{'*}_{K-2},
                     \mathbf{\overline{s}}^{'*}_{K-2}) \\
         &   p_{\mathbf{a}^+, \mathbf{r}}(z^{'*}_{K-2} \mid 
                     \mathbf{\overline{s}}^{'*}_{K-2},
                     \mathbf{\overline{a}}_{K-3}^+,
                     \mathbf{\overline{r}}_{K-3}, 
                     \mathbf{\overline{z}}^{'*}_{K-3})   \\
         &  p_{\mathbf{a}^+, \mathbf{r}}(s^{'*}_{K-2} \mid 
                     \mathbf{\overline{a}}_{K-3}^+,
                     \mathbf{\overline{r}}_{K-3}, 
                     \mathbf{\overline{z}}^{'*}_{K-3K-3},
                     \mathbf{\overline{s}}^{'*}_{K-3}) \\
\end{pmatrix*} \\
=         & p_{\mathbf{a}^+, \mathbf{r}}(y \mid
                     \mathbf{\overline{z}}^{'*}_{K},
                     \mathbf{\overline{s}}^{'*}_{K-3},
                     \mathbf{\overline{a}}_{K-3}^+,
                     \mathbf{\overline{r}}_{K-3}) \\
        &   p_{\mathbf{a}^+, \mathbf{r}}(a_{K-1}, r_{K-1} \mid
                     \mathbf{\overline{z}}^{'*}_{K-1},
                     \mathbf{\overline{s}}^{'*}_{K-3},
                     \mathbf{\overline{a}}_{K-3}^+,
                     \mathbf{\overline{r}}_{K-3}) \\            
        &   p_{\mathbf{a}^+, \mathbf{r}}(a_{K-2}, r_{K-2} \mid
                     \mathbf{\overline{z}}^{'*}_{K-2},
                     \mathbf{\overline{s}}^{'*}_{K-3},
                     \mathbf{\overline{a}}_{K-3}^+,
                     \mathbf{\overline{r}}_{K-3}) \\ 
& \sum\limits_{s^{'*}_{K-2}}  
         \begin{pmatrix*}[l] 
        &   p_{\mathbf{a}^+, \mathbf{r}}(a_{K}, r_K, \underline{\mathbf{z}}^{'*}_{K-2} ,s^{'*}_{K-2} \mid 
                     \mathbf{\overline{a}}_{K-3}^+,
                     \mathbf{\overline{r}}_{K-3}, 
                     \mathbf{\overline{z}}^{'*}_{K-3},
                     \mathbf{\overline{s}}^{'*}_{K-3}) \\
\end{pmatrix*} \\
=         & p_{\mathbf{a}^+, \mathbf{r}}(y \mid
                     \mathbf{\overline{z}}^{'*}_{K},
                     \mathbf{\overline{s}}^{'*}_{K-3},
                     \mathbf{\overline{a}}_{K-4}^+,
                     \mathbf{\overline{r}}_{K-4}) \\
        &   p_{\mathbf{a}^+, \mathbf{r}}(a_{K-1}, r_{K-1} \mid
                     \mathbf{\overline{z}}^{'*}_{K-1},
                     \mathbf{\overline{s}}^{'*}_{K-3},
                     \mathbf{\overline{a}}_{K-4}^+,
                     \mathbf{\overline{r}}_{K-4}) \\            
        &   p_{\mathbf{a}^+, \mathbf{r}}(a_{K-2}, r_{K-2} \mid
                     \mathbf{\overline{z}}^{'*}_{K-2},
                     \mathbf{\overline{s}}^{'*}_{K-3},
                     \mathbf{\overline{a}}_{K-4}^+,
                     \mathbf{\overline{r}}_{K-4}) \\ 
        &   p_{\mathbf{a}^+, \mathbf{r}}(a_{K}, r_K, \underline{\mathbf{z}}^{'*}_{K-2}  \mid 
                     \mathbf{\overline{a}}_{K-4}^+,
                     \mathbf{\overline{r}}_{K-4}, 
                     \mathbf{\overline{z}}^{'*}_{K-3},
                     \mathbf{\overline{s}}^{'*}_{K-3}) \\
=         & p_{\mathbf{a}^+, \mathbf{r}}(a_{K}, r_K \mid
                     \mathbf{\overline{z}}^{'*}_{K},
                     \mathbf{\overline{s}}^{'*}_{K-3},
                     \mathbf{\overline{a}}_{K-4}^+,
                     \mathbf{\overline{r}}_{K-4}) \\
        &   p_{\mathbf{a}^+, \mathbf{r}}(a_{K-1}, r_{K-1} \mid
                     \mathbf{\overline{z}}^{'*}_{K-1},
                     \mathbf{\overline{s}}^{'*}_{K-3},
                     \mathbf{\overline{a}}_{K-4}^+,
                     \mathbf{\overline{r}}_{K-4}) \\            
        &   p_{\mathbf{a}^+, \mathbf{r}}(a_{K-2}, r_{K-2} \mid
                     \mathbf{\overline{z}}^{'*}_{K-2},
                     \mathbf{\overline{s}}^{'*}_{K-3},
                     \mathbf{\overline{a}}_{K-4}^+,
                     \mathbf{\overline{r}}_{K-4}) \\ 
        &   p_{\mathbf{a}^+, \mathbf{r}}(y, \underline{\mathbf{z}}^{'*}_{K-2}  \mid 
                     \mathbf{\overline{a}}_{K-4}^+,
                     \mathbf{\overline{r}}_{K-4}, 
                     \mathbf{\overline{z}}^{'*}_{K-3},
                     \mathbf{\overline{s}}^{'*}_{K-3}) \\
\end{align*}

Under $(K-2)(iii)$ we have:

\begin{align*}
=         & p_{\mathbf{a}^+, \mathbf{r}}(y \mid
                     \mathbf{\overline{z}}^{'*}_{K},
                     \mathbf{\overline{s}}^{'*}_{K-3},
                     \mathbf{\overline{a}}_{K-3}^+,
                     \mathbf{\overline{r}}_{K-3}) \\
        &   p_{\mathbf{a}^+, \mathbf{r}}(a_{K}, r_K \mid 
                     \mathbf{\overline{a}}_{K-3}^+,
                     \mathbf{\overline{r}}_{K-3}, 
                     \mathbf{\overline{z}}^{'*}_{K},
                     \mathbf{\overline{s}}^{'*}_{K-3}) \\
        &   p_{\mathbf{a}^+, \mathbf{r}}(z^{'*}_{K} \mid 
                     \mathbf{\overline{a}}_{K-3}^+,
                     \mathbf{\overline{r}}_{K-3}, 
                     \mathbf{\overline{z}}^{'*}_{K-1},
                     \mathbf{\overline{s}}^{'*}_{K-3}) \\
        &   p_{\mathbf{a}^+, \mathbf{r}}(a_{K-2}, r_{K-2} \mid
                     \mathbf{\overline{z}}^{'*}_{K-2},
                     \mathbf{\overline{s}}^{'*}_{K-3},
                     \mathbf{\overline{a}}_{K-3}^+,
                     \mathbf{\overline{r}}_{K-3}) \\ 
& \sum\limits_{s^{'*}_{K-2}}  
         \begin{pmatrix*}[l] 
        &   p_{\mathbf{a}^+, \mathbf{r}}(a_{K-1}, r_{K-1} \mid
                     \mathbf{\overline{z}}^{'*}_{K-1},
                     \mathbf{\overline{s}}^{'*}_{K-2},
                     \mathbf{\overline{a}}_{K-3}^+,
                     \mathbf{\overline{r}}_{K-3}) \\ 
        &   p_{\mathbf{a}^+, \mathbf{r}}(z^{'*}_{K-1} \mid 
                     \mathbf{\overline{a}}_{K-3}^+,
                     \mathbf{\overline{r}}_{K-3}, 
                     \mathbf{\overline{z}}^{'*}_{K-2},
                     \mathbf{\overline{s}}^{'*}_{K-2}) \\
         &   p_{\mathbf{a}^+, \mathbf{r}}(z^{'*}_{K-2} \mid 
                     \mathbf{\overline{s}}^{'*}_{K-2},
                     \mathbf{\overline{a}}_{K-3}^+,
                     \mathbf{\overline{r}}_{K-3}, 
                     \mathbf{\overline{z}}^{'*}_{K-3})   \\
         &  p_{\mathbf{a}^+, \mathbf{r}}(s^{'*}_{K-2} \mid 
                     \mathbf{\overline{a}}_{K-3}^+,
                     \mathbf{\overline{r}}_{K-3}, 
                     \mathbf{\overline{z}}^{'*}_{K-3K-3},
                     \mathbf{\overline{s}}^{'*}_{K-3}) \\
\end{pmatrix*} \\
=         & p_{\mathbf{a}^+, \mathbf{r}}(y \mid
                     \mathbf{\overline{z}}^{'*}_{K},
                     \mathbf{\overline{s}}^{'*}_{K-3},
                     \mathbf{\overline{a}}_{K-3}^+,
                     \mathbf{\overline{r}}_{K-3}) \\
        &   p_{\mathbf{a}^+, \mathbf{r}}(a_{K}, r_K \mid 
                     \mathbf{\overline{a}}_{K-3}^+,
                     \mathbf{\overline{r}}_{K-3}, 
                     \mathbf{\overline{z}}^{'*}_{K},
                     \mathbf{\overline{s}}^{'*}_{K-3}) \\
        &   p_{\mathbf{a}^+, \mathbf{r}}(z^{'*}_{K} \mid 
                     \mathbf{\overline{a}}_{K-3}^+,
                     \mathbf{\overline{r}}_{K-3}, 
                     \mathbf{\overline{z}}^{'*}_{K-1},
                     \mathbf{\overline{s}}^{'*}_{K-3}) \\
        &   p_{\mathbf{a}^+, \mathbf{r}}(a_{K-2}, r_{K-2} \mid
                     \mathbf{\overline{z}}^{'*}_{K-2},
                     \mathbf{\overline{s}}^{'*}_{K-3},
                     \mathbf{\overline{a}}_{K-3}^+,
                     \mathbf{\overline{r}}_{K-3}) \\ 
& \sum\limits_{s^{'*}_{K-2}}  
         \begin{pmatrix*}[l] 
        &   p_{\mathbf{a}^+, \mathbf{r}}(a_{K-1}, r_{K-1}, z^{'*}_{K-1},z^{'*}_{K-2}, s^{'*}_{K-2} \mid 
                     \mathbf{\overline{a}}_{K-3}^+,
                     \mathbf{\overline{r}}_{K-3}, 
                     \mathbf{\overline{z}}^{'*}_{K-3},
                     \mathbf{\overline{s}}^{'*}_{K-3}) \\
\end{pmatrix*} \\
=         & p_{\mathbf{a}^+, \mathbf{r}}(y \mid
                     \mathbf{\overline{z}}^{'*}_{K},
                     \mathbf{\overline{s}}^{'*}_{K-3},
                     \mathbf{\overline{a}}_{K-4}^+,
                     \mathbf{\overline{r}}_{K-4}) \\
        &   p_{\mathbf{a}^+, \mathbf{r}}(a_{K}, r_K \mid 
                     \mathbf{\overline{a}}_{K-4}^+,
                     \mathbf{\overline{r}}_{K-4}, 
                     \mathbf{\overline{z}}^{'*}_{K},
                     \mathbf{\overline{s}}^{'*}_{K-3}) \\
        &   p_{\mathbf{a}^+, \mathbf{r}}(z^{'*}_{K} \mid 
                     \mathbf{\overline{a}}_{K-4}^+,
                     \mathbf{\overline{r}}_{K-4}, 
                     \mathbf{\overline{z}}^{'*}_{K-1},
                     \mathbf{\overline{s}}^{'*}_{K-3}) \\
        &   p_{\mathbf{a}^+, \mathbf{r}}(a_{K-2}, r_{K-2} \mid
                     \mathbf{\overline{z}}^{'*}_{K-2},
                     \mathbf{\overline{s}}^{'*}_{K-3},
                     \mathbf{\overline{a}}_{K-4}^+,
                     \mathbf{\overline{r}}_{K-4}) \\ 
        &   p_{\mathbf{a}^+, \mathbf{r}}(a_{K-1}, r_{K-1}, z^{'*}_{K-1},z^{'*}_{K-2} \mid 
                     \mathbf{\overline{a}}_{K-4}^+,
                     \mathbf{\overline{r}}_{K-4}, 
                     \mathbf{\overline{z}}^{'*}_{K-3},
                     \mathbf{\overline{s}}^{'*}_{K-3}) \\
=         & p_{\mathbf{a}^+, \mathbf{r}}(a_{K}, r_K \mid
                     \mathbf{\overline{z}}^{'*}_{K},
                     \mathbf{\overline{s}}^{'*}_{K-3},
                     \mathbf{\overline{a}}_{K-4}^+,
                     \mathbf{\overline{r}}_{K-4}) \\
        &   p_{\mathbf{a}^+, \mathbf{r}}(a_{K-1}, r_{K-1} \mid
                     \mathbf{\overline{z}}^{'*}_{K-1},
                     \mathbf{\overline{s}}^{'*}_{K-3},
                     \mathbf{\overline{a}}_{K-4}^+,
                     \mathbf{\overline{r}}_{K-4}) \\            
        &   p_{\mathbf{a}^+, \mathbf{r}}(a_{K-2}, r_{K-2} \mid
                     \mathbf{\overline{z}}^{'*}_{K-2},
                     \mathbf{\overline{s}}^{'*}_{K-3},
                     \mathbf{\overline{a}}_{K-4}^+,
                     \mathbf{\overline{r}}_{K-4}) \\ 
        &   p_{\mathbf{a}^+, \mathbf{r}}(y, \underline{\mathbf{z}}^{'*}_{K-2}  \mid 
                     \mathbf{\overline{a}}_{K-4}^+,
                     \mathbf{\overline{r}}_{K-4}, 
                     \mathbf{\overline{z}}^{'*}_{K-3},
                     \mathbf{\overline{s}}^{'*}_{K-3}) \\
\end{align*}

Thus under either $(K-2)(i)$ or $(K-2)(ii)$ or $(K-2)(iii)$ we have:

\begin{align*}
& \begin{pmatrix*}[l] 
    \sum\limits_{s^{'*}_{1}} & 
         \begin{pmatrix*}[l] 
     &   p(a_{1}, r_{1} \mid
                     \mathbf{\overline{z}}^{'*}_{1},
                     \mathbf{\overline{s}}^{'*}_{1}) \\
         &   p(z^{'*}_{1} \mid 
                     s^{'*}_{1})   \\
         &  p(s^{'*}_{1} ) \\ 
        & \vdots \\
&    \cdots \sum\limits_{s^{'*}_{K-3}}  \begin{pmatrix*}[l] 
& p_{\mathbf{a}^+, \mathbf{r}}(a_{K}, r_K \mid
                     \mathbf{\overline{z}}^{'*}_{K},
                     \mathbf{\overline{s}}^{'*}_{K-3},
                     \mathbf{\overline{a}}_{K-4}^+,
                     \mathbf{\overline{r}}_{K-4}) \\
        &   p_{\mathbf{a}^+, \mathbf{r}}(a_{K-1}, r_{K-1} \mid
                     \mathbf{\overline{z}}^{'*}_{K-1},
                     \mathbf{\overline{s}}^{'*}_{K-3},
                     \mathbf{\overline{a}}_{K-4}^+,
                     \mathbf{\overline{r}}_{K-4}) \\            
        &   p_{\mathbf{a}^+, \mathbf{r}}(a_{K-2}, r_{K-2} \mid
                     \mathbf{\overline{z}}^{'*}_{K-2},
                     \mathbf{\overline{s}}^{'*}_{K-3},
                     \mathbf{\overline{a}}_{K-4}^+,
                     \mathbf{\overline{r}}_{K-4}) \\ 
        &   p_{\mathbf{a}^+, \mathbf{r}}(y, \underline{\mathbf{z}}^{'*}_{K-2}  \mid 
                     \mathbf{\overline{a}}_{K-4}^+,
                     \mathbf{\overline{r}}_{K-4}, 
                     \mathbf{\overline{z}}^{'*}_{K-3},
                     \mathbf{\overline{s}}^{'*}_{K-3}) 
\end{pmatrix*}
\end{pmatrix*}
\end{pmatrix*}.
\end{align*}

 This concludes our consideration of the base case.

\underline{\textbf{The inductive step:}} We now show the equality in expression \eqref{eq: mainlemma} for $m=j$, assuming that it holds for all $m>j$ (for $j=K, K-1, K-2,\ldots)$. 

Thus, consider time point $j$:
 
 \begin{align*}
& \sum\limits_{s^{'*}_{j}}  
         \begin{pmatrix*}[l] 
&   p_{\mathbf{a}^+, \mathbf{r}}(y \mid 
                     \mathbf{\overline{a}}_{j-1}^+,
                     \mathbf{\overline{r}}_{j-1}, 
                     \mathbf{\overline{z}}^{'*}_{K},
                     \mathbf{\overline{s}}^{'*}_{j}) \\
  \prod\limits_{m=j+1}^{K} &  \begin{Bmatrix*}[l]
& p_{\mathbf{a}^+, \mathbf{r}}(a_{m},r_{m} \mid
                     \mathbf{\overline{z}}^{'*}_{m},
                     \mathbf{\overline{s}}^{'*}_{j},
                     \mathbf{\overline{a}}_{j-1}^+,
                     \mathbf{\overline{r}}_{j-1}) \\
& p_{\mathbf{a}^+, \mathbf{r}}(z^{'*}_{m} \mid
                     \mathbf{\overline{s}}^{'*}_{j},
                     \mathbf{\overline{a}}_{j-1}^+,
                     \mathbf{\overline{r}}_{j-1}) \\
\end{Bmatrix*} \\
         &   p(a_{j},r_{j} \mid
                     \mathbf{\overline{z}}^{'*}_{j},
                     \mathbf{\overline{s}}^{'*}_{j},
                     \mathbf{\overline{a}}_{j-1}^+,
                     \mathbf{\overline{r}}_{j-1}) \\
         &   p(z^{'*}_{j} \mid 
                     \mathbf{\overline{s}}^{'*}_{j},
                     \mathbf{\overline{a}}_{j-1}^+,
                     \mathbf{\overline{r}}_{j-1}, 
                     \mathbf{\overline{z}}^{'*}_{j-1})   \\
         &  p(s^{'*}_{j} \mid 
                     \mathbf{\overline{a}}_{j-1}^+,
                     \mathbf{\overline{r}}_{j-1}, 
                     \mathbf{\overline{z}}^{'*}_{j-1},
                     \mathbf{\overline{s}}^{'*}_{j-1})
\end{pmatrix*} \\
= & \sum\limits_{s^{'*}_{j}}  
         \begin{pmatrix*}[l] 
&   p_{\mathbf{a}^+, \mathbf{r}}(y \mid 
                     \mathbf{\overline{a}}_{j-1}^+,
                     \mathbf{\overline{r}}_{j-1}, 
                     \mathbf{\overline{z}}^{'*}_{K},
                     \mathbf{\overline{s}}^{'*}_{j}) \\
  \prod\limits_{m=j+1}^{K} &  \begin{Bmatrix*}[l]
& p_{\mathbf{a}^+, \mathbf{r}}(a_{m}, r_{m} \mid
                     \mathbf{\overline{z}}^{'*}_{m},
                     \mathbf{\overline{s}}^{'*}_{j},
                     \mathbf{\overline{a}}_{j-1}^+,
                     \mathbf{\overline{r}}_{j-1}) \\
& p_{\mathbf{a}^+, \mathbf{r}}(z^{'*}_{m} \mid
                     \mathbf{\overline{s}}^{'*}_{j},
                     \mathbf{\overline{a}}_{j-1}^+,
                     \mathbf{\overline{r}}_{j-1}) \\
\end{Bmatrix*} \\
         &   p_{\mathbf{a}^+, \mathbf{r}}(a_{j},r_{j} \mid
                     \mathbf{\overline{z}}^{'*}_{j},
                     \mathbf{\overline{s}}^{'*}_{j},
                     \mathbf{\overline{a}}_{j-1}^+,
                     \mathbf{\overline{r}}_{j-1}) \\
         &   p_{\mathbf{a}^+, \mathbf{r}}(z^{'*}_{j} \mid 
                     \mathbf{\overline{s}}^{'*}_{j},
                     \mathbf{\overline{a}}_{j-1}^+,
                     \mathbf{\overline{r}}_{j-1}, 
                     \mathbf{\overline{z}}^{'*}_{j-1})   \\
         &  p_{\mathbf{a}^+, \mathbf{r}}(s^{'*}_{j} \mid 
                     \mathbf{\overline{a}}_{j-1}^+,
                     \mathbf{\overline{r}}_{j-1}, 
                     \mathbf{\overline{z}}^{'*}_{j-1},
                     \mathbf{\overline{s}}^{'*}_{j-1})
\end{pmatrix*} \\
\end{align*}

As we saw in for the base-case with $m=K-1$, our proof techniques revolve around the following types of conditional independencies (justified by Lemma \ref{lemma: indgenlemma}):

\begin{align*}
    \Big( \mathbb{A}_{j} (\mathbf{a^{\dagger}}, \mathbf{r}), \mathbb{R}_{j} (\mathbf{a^{\dagger}}, \mathbf{r}) \Big)
        \CI 
            \mathbb{S}_{j}(\mathbf{a^{\dagger}}, \mathbf{r})
        \mid
            \overline{\mathbb{Z}}^{'*}_{j}(\mathbf{a^{\dagger}}, \mathbf{r}), 
            \overline{\mathbb{S}}^{'*}_{j-1}(\mathbf{a^{\dagger}}, \mathbf{r}),
            \overline{\mathbb{A}}_{j-1}(\mathbf{a^{\dagger}}, \mathbf{r}),
            \overline{\mathbb{R}}_{j-1}(\mathbf{a^{\dagger}}, \mathbf{r}), 
    \end{align*}

and that one of the $(K-j-1)$ following sets independencies hold:

\begin{itemize}
    \item [$(j)(i)$] For all $m \in \{j+1,\dots, K\}$
    \begin{align*}
          \Big(\mathbb{A}_m (\mathbf{a^{\dagger}}, \mathbf{r}), \mathbb{R}_m (\mathbf{a^{\dagger}}, \mathbf{r})\Big)
        \CI &
            \mathbb{S}_{j}(\mathbf{a^{\dagger}}, \mathbf{r})
        \mid
            \overline{\mathbb{Z}}^{'*}_{m}(\mathbf{a^{\dagger}}, \mathbf{r}), 
            \overline{\mathbb{S}}^{'*}_{j-1}(\mathbf{a^{\dagger}}, \mathbf{r}),
            \overline{\mathbb{A}}_{j-1}(\mathbf{a^{\dagger}}, \mathbf{r}),
            \overline{\mathbb{R}}_{j-1}(\mathbf{a^{\dagger}}, \mathbf{r}),
    \end{align*}
    \item [$(j)(ii)$] For all $m \in \{j+1,\dots, K-1\}$
    \begin{align*}
          \Big(\mathbb{A}_m (\mathbf{a^{\dagger}}, \mathbf{r}), \mathbb{R}_m (\mathbf{a^{\dagger}}, \mathbf{r})\Big)
        \CI &
            \mathbb{S}_{j}(\mathbf{a^{\dagger}}, \mathbf{r})
        \mid
            \overline{\mathbb{Z}}^{'*}_{m}(\mathbf{a^{\dagger}}, \mathbf{r}), 
            \overline{\mathbb{S}}^{'*}_{j-1}(\mathbf{a^{\dagger}}, \mathbf{r}),
            \overline{\mathbb{A}}_{j-1}(\mathbf{a^{\dagger}}, \mathbf{r}),
            \overline{\mathbb{R}}_{j-1}(\mathbf{a^{\dagger}}, \mathbf{r}), \text{ and } \\
         \mathbb{Y} (\mathbf{a^{\dagger}}, \mathbf{r})
        \CI &
            \mathbb{S}_{j}(\mathbf{a^{\dagger}}, \mathbf{r})
        \mid
            \overline{\mathbb{Z}}^{'*}_{K}(\mathbf{a^{\dagger}}, \mathbf{r}), 
            \overline{\mathbb{S}}^{'*}_{j-1}(\mathbf{a^{\dagger}}, \mathbf{r}),
            \overline{\mathbb{A}}_{j-1}(\mathbf{a^{\dagger}}, \mathbf{r}),
            \overline{\mathbb{R}}_{j-1}(\mathbf{a^{\dagger}}, \mathbf{r})
    \end{align*}
\item [$(j)(s)$]  $\forall 3 \leq s<K-j+1$: For all $m \in \{j+1,\dots, K-s+1, K-s+3, \dots, K\}$
    \begin{align*}
          \Big(\mathbb{A}_m (\mathbf{a^{\dagger}}, \mathbf{r}), \mathbb{R}_m (\mathbf{a^{\dagger}}, \mathbf{r})\Big)
        \CI &
            \mathbb{S}_{j}(\mathbf{a^{\dagger}}, \mathbf{r})
        \mid
            \overline{\mathbb{Z}}^{'*}_{m}(\mathbf{a^{\dagger}}, \mathbf{r}), 
            \overline{\mathbb{S}}^{'*}_{j-1}(\mathbf{a^{\dagger}}, \mathbf{r}),
            \overline{\mathbb{A}}_{j-1}(\mathbf{a^{\dagger}}, \mathbf{r}),
            \overline{\mathbb{R}}_{j-1}(\mathbf{a^{\dagger}}, \mathbf{r}), \text{ and } \\
         \mathbb{Y} (\mathbf{a^{\dagger}}, \mathbf{r})
        \CI &
            \mathbb{S}_{j}(\mathbf{a^{\dagger}}, \mathbf{r})
        \mid
            \overline{\mathbb{Z}}^{'*}_{K}(\mathbf{a^{\dagger}}, \mathbf{r}), 
            \overline{\mathbb{S}}^{'*}_{j-1}(\mathbf{a^{\dagger}}, \mathbf{r}),
            \overline{\mathbb{A}}_{j-1}(\mathbf{a^{\dagger}}, \mathbf{r}),
            \overline{\mathbb{R}}_{j-1}(\mathbf{a^{\dagger}}, \mathbf{r}), \text{ and } 
    \end{align*}   
  for all $r \in \{K-s+3, \dots, K\}$,   
        \begin{align*}
    \mathbb{Z}^{'*}_r (\mathbf{a^{\dagger}}, \mathbf{r})
        \CI &
            \mathbb{S}_{j}(\mathbf{a^{\dagger}}, \mathbf{r})
        \mid
            \overline{\mathbb{Z}}^{'*}_{r-1}(\mathbf{a^{\dagger}}, \mathbf{r}), 
            \overline{\mathbb{S}}^{'*}_{j-1}(\mathbf{a^{\dagger}}, \mathbf{r}),
            \overline{\mathbb{A}}_{j-1}(\mathbf{a^{\dagger}}, \mathbf{r}),
            \overline{\mathbb{R}}_{j-1}(\mathbf{a^{\dagger}}, \mathbf{r}). 
    \end{align*}   
\item [$\vdots$]
\item [$\vdots$]    
\item [$(j)(K-j+1)$]  For all $m \in \{j+2,\dots, K\}$
    \begin{align*}
          \Big(\mathbb{A}_m (\mathbf{a^{\dagger}}, \mathbf{r}), \mathbb{R}_m (\mathbf{a^{\dagger}}, \mathbf{r})\Big)
        \CI &
            \mathbb{S}_{j}(\mathbf{a^{\dagger}}, \mathbf{r})
        \mid
            \overline{\mathbb{Z}}^{'*}_{m}(\mathbf{a^{\dagger}}, \mathbf{r}), 
            \overline{\mathbb{S}}^{'*}_{j-1}(\mathbf{a^{\dagger}}, \mathbf{r}),
            \overline{\mathbb{A}}_{j-1}(\mathbf{a^{\dagger}}, \mathbf{r}),
            \overline{\mathbb{R}}_{j-1}(\mathbf{a^{\dagger}}, \mathbf{r}), \text{ and } \\
         \mathbb{Y} (\mathbf{a^{\dagger}}, \mathbf{r})
        \CI &
            \mathbb{S}_{j}(\mathbf{a^{\dagger}}, \mathbf{r})
        \mid
            \overline{\mathbb{Z}}^{'*}_{K}(\mathbf{a^{\dagger}}, \mathbf{r}), 
            \overline{\mathbb{S}}^{'*}_{j-1}(\mathbf{a^{\dagger}}, \mathbf{r}),
            \overline{\mathbb{A}}_{j-1}(\mathbf{a^{\dagger}}, \mathbf{r}),
            \overline{\mathbb{R}}_{j-1}(\mathbf{a^{\dagger}}, \mathbf{r}), \text{ and } 
    \end{align*}   
  for all $r \in \{j+2, \dots, K\}$,   
        \begin{align*}
    \mathbb{Z}^{'*}_r (\mathbf{a^{\dagger}}, \mathbf{r})
        \CI &
            \mathbb{S}_{j}(\mathbf{a^{\dagger}}, \mathbf{r})
        \mid
            \overline{\mathbb{Z}}^{'*}_{r-1}(\mathbf{a^{\dagger}}, \mathbf{r}), 
            \overline{\mathbb{S}}^{'*}_{j-1}(\mathbf{a^{\dagger}}, \mathbf{r}),
            \overline{\mathbb{A}}_{j-1}(\mathbf{a^{\dagger}}, \mathbf{r}),
            \overline{\mathbb{R}}_{j-1}(\mathbf{a^{\dagger}}, \mathbf{r}). 
    \end{align*}
\end{itemize}

Under $(j)(i)$ we have:

\begin{align*}
= & \prod\limits_{m=j}^{K}  
 p_{\mathbf{a}^+, \mathbf{r}}(a_{m}, r_{m} \mid
                     \mathbf{\overline{z}}^{'*}_{m},
                     \mathbf{\overline{s}}^{'*}_{j-1},
                     \mathbf{\overline{a}}_{j-1}^+,
                     \mathbf{\overline{r}}_{j-1})  \\
 \sum\limits_{s^{'*}_{j}}  &
         \begin{pmatrix*}[l] 
&   p_{\mathbf{a}^+, \mathbf{r}}(y \mid 
                     \mathbf{\overline{a}}_{j-1}^+,
                     \mathbf{\overline{r}}_{j-1}, 
                     \mathbf{\overline{z}}^{'*}_{K},
                     \mathbf{\overline{s}}^{'*}_{j}) \\
  \prod\limits_{m=j}^{K}  
& p_{\mathbf{a}^+, \mathbf{r}}(z^{'*}_{m} \mid
                     \mathbf{\overline{s}}^{'*}_{j},
                     \mathbf{\overline{a}}_{j-1}^+,
                     \mathbf{\overline{r}}_{j-1})  \\
         &  p_{\mathbf{a}^+, \mathbf{r}}(s^{'*}_{j} \mid 
                     \mathbf{\overline{a}}_{j-1}^+,
                     \mathbf{\overline{r}}_{j-1}, 
                     \mathbf{\overline{z}}^{'*}_{j-1},
                     \mathbf{\overline{s}}^{'*}_{j-1})
\end{pmatrix*} \\
= & \prod\limits_{m=j}^{K}  
 p_{\mathbf{a}^+, \mathbf{r}}(a_{m}, r_{m} \mid
                     \mathbf{\overline{z}}^{'*}_{m},
                     \mathbf{\overline{s}}^{'*}_{j-1},
                     \mathbf{\overline{a}}_{j-1}^+,
                     \mathbf{\overline{r}}_{j-1})  \\
 \sum\limits_{s^{'*}_{j}}  &
         \begin{pmatrix*}[l] 
&   p_{\mathbf{a}^+, \mathbf{r}}(y, \underline{\mathbf{z}}^{'*}_j, s^{'*}_{j} \mid 
                     \mathbf{\overline{a}}_{j-1}^+,
                     \mathbf{\overline{r}}_{j-1}, 
                     \mathbf{\overline{z}}^{'*}_{j-1},
                     \mathbf{\overline{s}}^{'*}_{j-1})
\end{pmatrix*} \\
= & \prod\limits_{m=j}^{K}  
 p_{\mathbf{a}^+, \mathbf{r}}(a_{m}, r_{m} \mid
                     \mathbf{\overline{z}}^{'*}_{m},
                     \mathbf{\overline{s}}^{'*}_{j-1},
                     \mathbf{\overline{a}}_{j-2}^+,
                     \mathbf{\overline{r}}_{j-2})  \\
&   p_{\mathbf{a}^+, \mathbf{r}}(y, \underline{\mathbf{z}}^{'*}_j \mid 
                     \mathbf{\overline{a}}_{j-2}^+,
                     \mathbf{\overline{r}}_{j-2}, 
                     \mathbf{\overline{z}}^{'*}_{j-1},
                     \mathbf{\overline{s}}^{'*}_{j-1})
\end{align*}

Under $(j)(s)$ we have:

\begin{align*}
=  \prod\limits_{\{m\ge j, m\neq K-s+2\}}  &
 p_{\mathbf{a}^+, \mathbf{r}}(a_{m}, r_{m} \mid
                     \mathbf{\overline{z}}^{'*}_{m},
                     \mathbf{\overline{s}}^{'*}_{j-1},
                     \mathbf{\overline{a}}_{j-1}^+,
                     \mathbf{\overline{r}}_{j-1})  \\
&   p_{\mathbf{a}^+, \mathbf{r}}(y \mid 
                     \mathbf{\overline{a}}_{j-1}^+,
                     \mathbf{\overline{r}}_{j-1}, 
                     \mathbf{\overline{z}}^{'*}_{K},
                     \mathbf{\overline{s}}^{'*}_{j-1}) \\
 \prod\limits_{m=K-s+3}^{K}&
 p_{\mathbf{a}^+, \mathbf{r}}(z^{'*}_{m} \mid
                     \mathbf{\overline{s}}^{'*}_{j-1},
                     \mathbf{\overline{a}}_{j-1}^+,
                     \mathbf{\overline{r}}_{j-1})  \\
 \sum\limits_{s^{'*}_{j}}  &
         \begin{pmatrix*}[l] 
 &  p_{\mathbf{a}^+, \mathbf{r}}(a_{K-s+2}, r_{K-s+2} \mid
                     \mathbf{\overline{z}}^{'*}_{K-s+2},
                     \mathbf{\overline{s}}^{'*}_{j},
                     \mathbf{\overline{a}}_{j-1}^+,
                     \mathbf{\overline{r}}_{j-1}) \\       
  \prod\limits_{m=j}^{K-s+2}  
& p_{\mathbf{a}^+, \mathbf{r}}(z^{'*}_{m} \mid
                     \mathbf{\overline{s}}^{'*}_{j},
                     \mathbf{\overline{a}}_{j-1}^+,
                     \mathbf{\overline{r}}_{j-1})   \\
         &  p_{\mathbf{a}^+, \mathbf{r}}(s^{'*}_{j} \mid 
                     \mathbf{\overline{a}}_{j-1}^+,
                     \mathbf{\overline{r}}_{j-1}, 
                     \mathbf{\overline{z}}^{'*}_{j-1},
                     \mathbf{\overline{s}}^{'*}_{j-1})
\end{pmatrix*} \\
=  \prod\limits_{\{m\ge j, m\neq K-s+2\}}  &
 p_{\mathbf{a}^+, \mathbf{r}}(a_{m}, r_{m} \mid
                     \mathbf{\overline{z}}^{'*}_{m},
                     \mathbf{\overline{s}}^{'*}_{j-1},
                     \mathbf{\overline{a}}_{j-1}^+,
                     \mathbf{\overline{r}}_{j-1})  \\
&   p_{\mathbf{a}^+, \mathbf{r}}(y \mid 
                     \mathbf{\overline{a}}_{j-1}^+,
                     \mathbf{\overline{r}}_{j-1}, 
                     \mathbf{\overline{z}}^{'*}_{K},
                     \mathbf{\overline{s}}^{'*}_{j-1}) \\
 \prod\limits_{m=K-s+3}^{K}&
 p_{\mathbf{a}^+, \mathbf{r}}(z^{'*}_{m} \mid
                     \mathbf{\overline{s}}^{'*}_{j-1},
                     \mathbf{\overline{a}}_{j-1}^+,
                     \mathbf{\overline{r}}_{j-1})  \\
 \sum\limits_{s^{'*}_{j}}  &
         \begin{pmatrix*}[l] 
 &  p_{\mathbf{a}^+, \mathbf{r}}(a_{K-s+2}, r_{K-s+2}, z^{'*}_{K-s+2}, \dots, z^{'*}_{j}, s^{'*}_{j} \mid 
                     \mathbf{\overline{a}}_{j-1}^+,
                     \mathbf{\overline{r}}_{j-1}, 
                     \mathbf{\overline{z}}^{'*}_{j-1},
                     \mathbf{\overline{s}}^{'*}_{j-1})
\end{pmatrix*} \\
=  \prod\limits_{\{m\ge j, m\neq K-s+2\}}  &
 p_{\mathbf{a}^+, \mathbf{r}}(a_{m}, r_{m} \mid
                     \mathbf{\overline{z}}^{'*}_{m},
                     \mathbf{\overline{s}}^{'*}_{j-1},
                     \mathbf{\overline{a}}_{j-2}^+,
                     \mathbf{\overline{r}}_{j-2})  \\
&   p_{\mathbf{a}^+, \mathbf{r}}(y \mid 
                     \mathbf{\overline{a}}_{j-2}^+,
                     \mathbf{\overline{r}}_{j-2}, 
                     \mathbf{\overline{z}}^{'*}_{K},
                     \mathbf{\overline{s}}^{'*}_{j-1}) \\
 \prod\limits_{m=K-s+3}^{K}&
 p_{\mathbf{a}^+, \mathbf{r}}(z^{'*}_{m} \mid
                     \mathbf{\overline{s}}^{'*}_{j-1},
                     \mathbf{\overline{a}}_{j-2}^+,
                     \mathbf{\overline{r}}_{j-2})  \\
 &  p_{\mathbf{a}^+, \mathbf{r}}(a_{K-s+2}, r_{K-s+2}, z^{'*}_{K-s+2}, \dots, z^{'*}_{j} \mid 
                     \mathbf{\overline{a}}_{j-2}^+,
                     \mathbf{\overline{r}}_{j-2}, 
                     \mathbf{\overline{z}}^{'*}_{j-1},
                     \mathbf{\overline{s}}^{'*}_{j-1}) \\
=  \prod\limits_{m=j}^{K}  & 
 p_{\mathbf{a}^+, \mathbf{r}}(a_{m}, r_{m} \mid
                     \mathbf{\overline{z}}^{'*}_{m},
                     \mathbf{\overline{s}}^{'*}_{j-1},
                     \mathbf{\overline{a}}_{j-2}^+,
                     \mathbf{\overline{r}}_{j-2})  \\
&   p_{\mathbf{a}^+, \mathbf{r}}(y, \underline{\mathbf{z}}^{'*}_j \mid 
                     \mathbf{\overline{a}}_{j-2}^+,
                     \mathbf{\overline{r}}_{j-2}, 
                     \mathbf{\overline{z}}^{'*}_{j-1},
                     \mathbf{\overline{s}}^{'*}_{j-1})
\end{align*}

Under $(j)(K-j-1)$ we have:

 \begin{align*}
=  \prod\limits_{\{m\ge j, m\neq j+1\}}  &
 p_{\mathbf{a}^+, \mathbf{r}}(a_{m}, r_{m} \mid
                     \mathbf{\overline{z}}^{'*}_{m},
                     \mathbf{\overline{s}}^{'*}_{j-1},
                     \mathbf{\overline{a}}_{j-1}^+,
                     \mathbf{\overline{r}}_{j-1})  \\
&   p_{\mathbf{a}^+, \mathbf{r}}(y \mid 
                     \mathbf{\overline{a}}_{j-1}^+,
                     \mathbf{\overline{r}}_{j-1}, 
                     \mathbf{\overline{z}}^{'*}_{K},
                     \mathbf{\overline{s}}^{'*}_{j-1}) \\
 \prod\limits_{m=j+2}^{K}&
 p_{\mathbf{a}^+, \mathbf{r}}(z^{'*}_{m} \mid
                     \mathbf{\overline{s}}^{'*}_{j-1},
                     \mathbf{\overline{a}}_{j-1}^+,
                     \mathbf{\overline{r}}_{j-1})  \\
 \sum\limits_{s^{'*}_{j}}  &
         \begin{pmatrix*}[l] 
 &  p_{\mathbf{a}^+, \mathbf{r}}(a_{j+1}, r_{j+1} \mid
                     \mathbf{\overline{z}}^{'*}_{j+1},
                     \mathbf{\overline{s}}^{'*}_{j},
                     \mathbf{\overline{a}}_{j-1}^+,
                     \mathbf{\overline{r}}_{j-1}) \\       
  \prod\limits_{m=j}^{j+1}  
& p_{\mathbf{a}^+, \mathbf{r}}(z^{'*}_{m} \mid
                     \mathbf{\overline{s}}^{'*}_{j},
                     \mathbf{\overline{a}}_{j-1}^+,
                     \mathbf{\overline{r}}_{j-1})   \\
         &  p_{\mathbf{a}^+, \mathbf{r}}(s^{'*}_{j} \mid 
                     \mathbf{\overline{a}}_{j-1}^+,
                     \mathbf{\overline{r}}_{j-1}, 
                     \mathbf{\overline{z}}^{'*}_{j-1},
                     \mathbf{\overline{s}}^{'*}_{j-1})
\end{pmatrix*} \\
=  \prod\limits_{\{m\ge j, m\neq j+1\}}  &
 p_{\mathbf{a}^+, \mathbf{r}}(a_{m}, r_{m} \mid
                     \mathbf{\overline{z}}^{'*}_{m},
                     \mathbf{\overline{s}}^{'*}_{j-1},
                     \mathbf{\overline{a}}_{j-1}^+,
                     \mathbf{\overline{r}}_{j-1})  \\
&   p_{\mathbf{a}^+, \mathbf{r}}(y \mid 
                     \mathbf{\overline{a}}_{j-1}^+,
                     \mathbf{\overline{r}}_{j-1}, 
                     \mathbf{\overline{z}}^{'*}_{K},
                     \mathbf{\overline{s}}^{'*}_{j-1}) \\
 \prod\limits_{m=j+2}^{K}&
 p_{\mathbf{a}^+, \mathbf{r}}(z^{'*}_{m} \mid
                     \mathbf{\overline{s}}^{'*}_{j-1},
                     \mathbf{\overline{a}}_{j-1}^+,
                     \mathbf{\overline{r}}_{j-1})  \\
 \sum\limits_{s^{'*}_{j}}  &
         \begin{pmatrix*}[l] 
 &  p_{\mathbf{a}^+, \mathbf{r}}(a_{j+1}, r_{j+1}, z^{'*}_{j+1}, z^{'*}_{j}, s^{'*}_{j} \mid 
                     \mathbf{\overline{a}}_{j-1}^+,
                     \mathbf{\overline{r}}_{j-1}, 
                     \mathbf{\overline{z}}^{'*}_{j-1},
                     \mathbf{\overline{s}}^{'*}_{j-1})
\end{pmatrix*} \\
=  \prod\limits_{\{m\ge j, m\neq j+1\}}  &
 p_{\mathbf{a}^+, \mathbf{r}}(a_{m}, r_{m} \mid
                     \mathbf{\overline{z}}^{'*}_{m},
                     \mathbf{\overline{s}}^{'*}_{j-1},
                     \mathbf{\overline{a}}_{j-2}^+,
                     \mathbf{\overline{r}}_{j-2})  \\
&   p_{\mathbf{a}^+, \mathbf{r}}(y \mid 
                     \mathbf{\overline{a}}_{j-2}^+,
                     \mathbf{\overline{r}}_{j-2}, 
                     \mathbf{\overline{z}}^{'*}_{K},
                     \mathbf{\overline{s}}^{'*}_{j-1}) \\
 \prod\limits_{m=j+2}^{K}&
 p_{\mathbf{a}^+, \mathbf{r}}(z^{'*}_{m} \mid
                     \mathbf{\overline{s}}^{'*}_{j-1},
                     \mathbf{\overline{a}}_{j-2}^+,
                     \mathbf{\overline{r}}_{j-2})  \\
 &  p_{\mathbf{a}^+, \mathbf{r}}(a_{j+1}, r_{j+1}, z^{'*}_{j+1}, z^{'*}_{j}\mid 
                     \mathbf{\overline{a}}_{j-2}^+,
                     \mathbf{\overline{r}}_{j-2}, 
                     \mathbf{\overline{z}}^{'*}_{j-1},
                     \mathbf{\overline{s}}^{'*}_{j-1}) \\
=  \prod\limits_{m=j}^{K}  & 
 p_{\mathbf{a}^+, \mathbf{r}}(a_{m}, r_{m} \mid
                     \mathbf{\overline{z}}^{'*}_{m},
                     \mathbf{\overline{s}}^{'*}_{j-1},
                     \mathbf{\overline{a}}_{j-2}^+,
                     \mathbf{\overline{r}}_{j-2})  \\
&   p_{\mathbf{a}^+, \mathbf{r}}(y, \underline{\mathbf{z}}^{'*}_j \mid 
                     \mathbf{\overline{a}}_{j-2}^+,
                     \mathbf{\overline{r}}_{j-2}, 
                     \mathbf{\overline{z}}^{'*}_{j-1},
                     \mathbf{\overline{s}}^{'*}_{j-1})
\end{align*}
 
Thus under either $(j)(i)$ or $(j)(ii)$ or $\dots (j)(K-j-1)$ we have:

\begin{align*}
    \sum\limits_{s^{'*}_{1}} & 
         \begin{pmatrix*}[l] 
     &   p(a_{1}, r_{1} \mid
                     \mathbf{\overline{z}}^{'*}_{1},
                     \mathbf{\overline{s}}^{'*}_{1}) \\
         &   p(z^{'*}_{1} \mid 
                     s^{'*}_{1})   \\
         &  p(s^{'*}_{1} ) \\ 
        & \vdots \\
&    \cdots  \sum\limits_{s^{'*}_{j-1}}  \begin{pmatrix*}[l] 
\prod\limits_{m=j}^{K}  & 
 p_{\mathbf{a}^+, \mathbf{r}}(a_{m}, r_{m} \mid
                     \mathbf{\overline{z}}^{'*}_{m},
                     \mathbf{\overline{s}}^{'*}_{j-1},
                     \mathbf{\overline{a}}_{j-2}^+,
                     \mathbf{\overline{r}}_{j-2})  \\
&   p_{\mathbf{a}^+, \mathbf{r}}(y, \underline{\mathbf{z}}^{'*}_j \mid 
                     \mathbf{\overline{a}}_{j-2}^+,
                     \mathbf{\overline{r}}_{j-2}, 
                     \mathbf{\overline{z}}^{'*}_{j-1},
                     \mathbf{\overline{s}}^{'*}_{j-1})
\end{pmatrix*}
\end{pmatrix*}.
\end{align*}

Taking $j=2$ we have:

\begin{align*}
\sum\limits_{\mathbf{a}', \mathbf{r}'} p_{\mathbf{a}^+}( \mathbf{z}) = &
 p_{\mathbf{a}^+, \mathbf{r}}(y, \underline{\mathbf{z}}^{'*}_1)
        \prod\limits_{m=1}^{K}   
         p_{\mathbf{a}^+, \mathbf{r}}(a_{m}, r_{m} \mid
                             \mathbf{\overline{z}}^{'*}_{m})  
           \\
= &       \underbrace{p_{\mathbf{a}^+}}_{(**)}(y, \underline{\mathbf{z}}^{'*}_1)  \prod\limits_{m=1}^{K}   
         p_{\mathbf{a}^+, \mathbf{r}}(a_{m}, r_{m} \mid
                             \mathbf{\overline{z}}^{'*}_{m}, \underbrace{\mathbf{\overline{r}}_{m-1}}_{(*)}) 
            \\
= &    p_{\mathbf{a}^+}(y, \underline{\mathbf{z}}^{'*}_1) 
        \prod\limits_{m=1}^{K}   
         \underbrace{p_{\mathbf{a}^*}}_{(*)}(a_{m}, r_{m} \mid
                             \mathbf{\overline{z}}^{'*}_{m}, \mathbf{\overline{r}}_{m-1})  
\end{align*}

In the above, the first equality follows by our inductive arguments, the second follows by Condition \eqref{eq: irrel1} (instrument irrelevance) and Lemma \ref{lemma: rstarex} (Reduced exchangeability for relevant instruments) combined with Lemma \ref{lemma: indgenlemma2} (collision impossibility for ancestors). The final equality follows by Lemma \ref{lemma49} (consistency).

This concludes the proof of Lemma \ref{lemma: mainlemma}.

We now continue our proof of Theorem \ref{thm: stochgform}.

\begin{align*}
   P(\mathbb{Z}'(g) =\mathbf{z'}) = & \\ \sum\limits_{\mathbf{a}, \mathbf{r}}P(\mathbb{Z}(g) = \mathbf{z}) = &  \sum\limits_{\mathbf{a}, \mathbf{r}}  \sum\limits_{\mathbf{a}^+,  \mathbf{s}}
        p(y\mid \mathbf{\overline{l}}_K, \mathbf{\overline{a}}_K^+)
        \prod\limits_{j=1}^{K}
        p(l_j, a_j \mid \mathbf{\overline{l}}_{j-1}, \mathbf{\overline{a}}_{j-1}^+)
        \prod\limits_{t=1}^{K}
        q_t^{g}(a_t^+ \mid \mathbf{pa}_t^+) \\
= &    \sum\limits_{\mathbf{a}^*, \mathbf{r}}\sum\limits_{\mathbf{a}^+} \Big\{\prod\limits_{t=1}^{K}
        q_t^{g}(a_t^+ \mid \mathbf{pa}_t^+)\Big\}\sum\limits_{\mathbf{a}', \mathbf{r}'} \sum\limits_{\mathbf{s}}
        p(y\mid \mathbf{\overline{l}}_K, \mathbf{\overline{a}}_K^+)
        \prod\limits_{j=1}^{K}
        p(l_j, a_j \mid \mathbf{\overline{l}}_{j-1}, \mathbf{\overline{a}}_{j-1}^+)
         \\
= &   \sum\limits_{\mathbf{a}^*, \mathbf{r}} \sum\limits_{\mathbf{a}^+} \Big\{\prod\limits_{t=1}^{K}
        q_t^{g}(a_t^+ \mid \mathbf{pa}_t^+)\Big\} p_{\mathbf{a}^+}(y, \underline{\mathbf{z}}^{'*}_1) 
        \prod\limits_{m=1}^{K}   
         p_{\mathbf{a}^*}(a_{m}, r_{m} \mid
                             \mathbf{\overline{z}}^{'*}_{m}, \mathbf{\overline{r}}_{m-1})
         \\
= &   \sum\limits_{\mathbf{a}^+} \Bigg\{ \sum\limits_{\mathbf{a}^*, \mathbf{r}}\prod\limits_{t=1}^{K}
        q_t^{g}(a_t^+ \mid \mathbf{pa}_t^+)\prod\limits_{m=1}^{K}   
         p_{\mathbf{a}^*}(a_{m}, r_{m} \mid
                             \mathbf{\overline{z}}^{'*}_{m}, \mathbf{\overline{r}}_{m-1})\Bigg\} b_{\mathbf{a}^+}(y, \underline{\mathbf{z}}^{'*}_1) 
         \\
= &  \sum\limits_{\mathbf{a}^+,  \mathbf{s'}}\Bigg\{\prod\limits_{t=1}^{K}
        \tilde{q}_t^{g}(a_t^+ \mid \mathbf{\overline{l}}'_{t}, \mathbf{\overline{a}}_{t-1}^+)\Bigg\}
        p(y\mid \mathbf{\overline{l}'}_K, \mathbf{\overline{a}}_K^+)
        \prod\limits_{j=1}^{K}
        p(l'_j \mid \mathbf{\overline{l}'}_{j-1}, \mathbf{\overline{a}}_{j-1}^+)
         \\
= & f^{g, \textbf{red}}(\mathbf{z'}).
\end{align*}

The first and second equalities follow by definition of $Z'$ and of the dynamic g-formula. The third follows since by definition $a'$ and $r'$ cannot be in $\mathbf{pa}_t^+$. The fourth follows by Lemma \ref{lemma: mainlemma}. The fifth rearranges terms and uses the definition of the multivariate g-formula. The final equalities follow by laws of probability and definitions of the reduced g-formula, thus concluding the proof of Theorem \ref{thm: stochgform}.

\end{proof}

\subsubsection{Proof of Propositions \ref{prop: stochgform1} and \ref{prop: stochgform2} and Corollary \ref{cor: stochgform}}

To prove Proposition \ref{prop: stochgform1}, consider the term $ p_{\mathbf{a}^+}( \mathbf{z})$, which we can re-write (as in the proof for Lemma \ref{lemma: mainlemma}) as follows:

\begin{align*}
 p_{\mathbf{a}^+}( \mathbf{z}) = \sum\limits_{s^{'*}_{1}} & 
         \begin{pmatrix*}[l] 
     &   p(a_{1}, r_{1} \mid
                     \mathbf{\overline{z}}^{'*}_{1},
                     \mathbf{\overline{s}}^{'*}_{1}) \\
         &   p(z^{'*}_{1} \mid 
                     s^{'*}_{1})   \\
         &  p(s^{'*}_{1} ) \\ 
        & \vdots \\
&    \cdots 
   \sum\limits_{s^{'*}_{m}}  
         \begin{pmatrix*}[l] 
         &   p(a_{m}, r_{m} \mid
                     \mathbf{\overline{z}}^{'*}_{m},
                     \mathbf{\overline{s}}^{'*}_{m},
                     \mathbf{\overline{a}}_{m-1}^+,
                     \mathbf{\overline{r}}_{m-1}) \\
         &   p(z^{'*}_{m} \mid 
                     \mathbf{\overline{s}}^{'*}_{m},
                     \mathbf{\overline{a}}_{m-1}^+,
                     \mathbf{\overline{r}}_{m-1}, 
                     \mathbf{\overline{z}}^{'*}_{m-1})   \\
         &  p(s^{'*}_{m} \mid 
                     \mathbf{\overline{a}}_{m-1}^+,
                     \mathbf{\overline{r}}_{m-1}, 
                     \mathbf{\overline{z}}^{'*}_{m-1},
                     \mathbf{\overline{s}}^{'*}_{m-1}) \\
       &  \vdots \\
 & \cdots  \sum\limits_{s^{'*}_{K}}                
            \begin{pmatrix*}[l]
                 &   p(y \mid 
                            \mathbf{\overline{a}}_{K}^+, 
                            \mathbf{\overline{r}}_{K}, 
                            \mathbf{\overline{z}}^{'*}_{K}, 
                            \mathbf{\overline{s}}^{'*}_{K}) \\
                 &   p(a_K, r_K \mid
                             \mathbf{\overline{z}}^{'*}_{K},
                             \mathbf{\overline{s}}^{'*}_{K},
                             \mathbf{\overline{a}}_{K-1}^+,
                             \mathbf{\overline{r}}_{K-1}) \\
                 &   p(z^{'*}_{K} \mid 
                             \mathbf{\overline{s}}^{'*}_{K},
                             \mathbf{\overline{a}}_{K-1}^+,
                             \mathbf{\overline{r}}_{K-1}, 
                             \mathbf{\overline{z}}^{'*}_{K-1})   \\
                 &  p(s^{'*}_{K} \mid 
                             \mathbf{\overline{a}}_{K-1}^+
                             \mathbf{\overline{r}}_{K-1}, 
                             \mathbf{\overline{z}}^{'*}_{K-1},
                             \mathbf{\overline{s}}^{'*}_{K-1}) 
            \end{pmatrix*}
\cdots
\end{pmatrix*}
\cdots
\end{pmatrix*}
\end{align*}

Consider each term of the form $p(z^{'*}_{m} \mid 
                     \mathbf{\overline{s}}^{'*}_{m},
                     \mathbf{\overline{a}}_{m-1}^+,
                     \mathbf{\overline{r}}_{m-1}, 
                     \mathbf{\overline{z}}^{'*}_{m-1})$:
                     
\begin{align*}
   & p(z^{'*}_{m} \mid 
                     \mathbf{\overline{s}}^{'*}_{m},
                     \mathbf{\overline{a}}_{m-1}^+,
                     \mathbf{\overline{r}}_{m-1}, 
                     \mathbf{\overline{z}}^{'*}_{m-1}) \\
=& p_{\mathbf{a}^+, \mathbf{r}}(z^{'*}_{m} \mid 
                     \mathbf{\overline{s}}^{'*}_{m},
                     \mathbf{\overline{a}}_{m-1}^+,
                     \mathbf{\overline{r}}_{m-1}, 
                     \mathbf{\overline{z}}^{'*}_{m-1}) \\
=& p_{\mathbf{a}^+, \mathbf{r}}(z^{'*}_{m} \mid 
                     \mathbf{\overline{s}}^{'*}_{m},
                     \mathbf{\overline{a}}_{m-1}^+,
                     \mathbf{\overline{z}}^{'*}_{m-1}) \\
=& p_{\mathbf{a}^+}(z^{'*}_{m} \mid 
                     \mathbf{\overline{s}}^{'*}_{m},
                     \mathbf{\overline{a}}_{m-1}^+,
                     \mathbf{\overline{z}}^{'*}_{m-1}) \\    
=& p(z^{'*}_{m} \mid 
                     \mathbf{\overline{s}}^{'*}_{m},
                     \mathbf{\overline{a}}_{m-1}^+,
                     \mathbf{\overline{z}}^{'*}_{m-1}).             .
\end{align*}

The first equality follows by Lemma \ref{lemma49} (consistency). The second by the sequential exchangeability condition \eqref{eq: irrelRb} of Proposition \ref{prop: stochgform1} and Lemma \ref{lemma: indgenlemma2} (collision impossibility for ancestors). The third follows by the instrumental irrelevance condition \eqref{eq: irrel2Rb} of Proposition \ref{prop: stochgform1}. The fourth follows by Lemma \ref{lemma49} (consistency). 

The conditions of Proposition \ref{prop: stochgform1} allow extension of these arguments to the density for $s^{'*}_{m}$ so we also have:

\begin{align*}
   & p(s^{'*}_{m} \mid 
                     \mathbf{\overline{a}}_{m-1}^+,
                     \mathbf{\overline{r}}_{m-1}, 
                     \mathbf{\overline{z}}^{'*}_{m-1},
                     \mathbf{\overline{s}}^{'*}_{m-1}) \\
=& p(s^{'*}_{m} \mid 
                     \mathbf{\overline{a}}_{m-1}^+,
                     \mathbf{\overline{z}}^{'*}_{m-1},
                     \mathbf{\overline{s}}^{'*}_{m-1}).            .
\end{align*}
                     
Then we can re-write $ p_{\mathbf{a}^+}( \mathbf{z})$:

\begin{align*}
 p_{\mathbf{a}^+}( \mathbf{z}) = \sum\limits_{\mathbf{s}}
        p(y\mid \mathbf{\overline{l}}'_K, \mathbf{\overline{a}}_K^+)
        \prod\limits_{j=1}^{K}
        p(l'_j \mid \mathbf{\overline{l}}'_{j-1}, \mathbf{\overline{a}}_{j-1}^+)
        \prod\limits_{j=1}^{K}
        p(a_j, r_j \mid \mathbf{\overline{l}}'_{j-1}, \mathbf{\overline{r}}_{j-1}, \mathbf{\overline{a}}_{j-1}^+)
\end{align*}

We now continue our proof of Proposition \ref{prop: stochgform1}.

\begin{align*}
   P(\mathbb{Z}'(g) =\mathbf{z'}) = & \\ \sum\limits_{\mathbf{a}, \mathbf{r}}P(\mathbb{Z}(g) = \mathbf{z}) = &  \sum\limits_{\mathbf{a}, \mathbf{r}}  \sum\limits_{\mathbf{a}^+,  \mathbf{s}}
        p(y\mid \mathbf{\overline{l}}_K, \mathbf{\overline{a}}_K^+)
        \prod\limits_{j=1}^{K}
        p(l_j, a_j \mid \mathbf{\overline{l}}_{j-1}, \mathbf{\overline{a}}_{j-1}^+)
        \prod\limits_{t=1}^{K}
        q_t^{g}(a_t^+ \mid \mathbf{pa}_t^+) \\
= &    \sum\limits_{\mathbf{a}^*, \mathbf{r}}\sum\limits_{\mathbf{a}^+} \Big\{\prod\limits_{t=1}^{K}
        q_t^{g}(a_t^+ \mid \mathbf{pa}_t^+)\Big\} p_{\mathbf{a}^+}( \mathbf{z})
         \\
= &    \sum\limits_{\mathbf{a}^*, \mathbf{r}}\sum\limits_{\mathbf{a}^+} \Big\{\prod\limits_{t=1}^{K}
        q_t^{g}(a_t^+ \mid \mathbf{pa}_t^+)\Big\} \sum\limits_{\mathbf{s}}
        p(y\mid \mathbf{\overline{l}}'_K, \mathbf{\overline{a}}_K^+)
        \prod\limits_{j=1}^{K}
        p(l'_j \mid \mathbf{\overline{l}}'_{j-1}, \mathbf{\overline{a}}_{j-1}^+)
        \prod\limits_{j=1}^{K}
        p(a_j, r_j \mid \mathbf{\overline{l}}'_{j-1}, \mathbf{\overline{r}}_{j-1}, \mathbf{\overline{a}}_{j-1}^+)
         \\
= &   \sum\limits_{\mathbf{a}^+} \Bigg\{ \sum\limits_{\mathbf{a}^*, \mathbf{r}}\prod\limits_{t=1}^{K}
        q_t^{g}(a_t^+ \mid \mathbf{pa}_t^+)\prod\limits_{m=1}^{K}   
         p(a_j, r_j \mid \mathbf{\overline{l}}'_{j-1}, \mathbf{\overline{r}}_{j-1}, \mathbf{\overline{a}}_{j-1}^+)\Bigg\} b_{\mathbf{a}^+}(y, \underline{\mathbf{z}}^{'*}_1) 
         \\
= &  \sum\limits_{\mathbf{a}^+,  \mathbf{s'}}\Bigg\{\prod\limits_{t=1}^{K}
        \tilde{q}_t^{g}(a_t^+ \mid \mathbf{\overline{l}}'_{t}, \mathbf{\overline{a}}_{t-1}^+)\Bigg\}
        p(y\mid \mathbf{\overline{l}'}_K, \mathbf{\overline{a}}_K^+)
        \prod\limits_{j=1}^{K}
        p(l'_j \mid \mathbf{\overline{l}'}_{j-1}, \mathbf{\overline{a}}_{j-1}^+)
\end{align*}

The first two equalities repeat those in the final panel for the proof of Theorem \ref{thm: stochgform}. The third equality follows by arguments made immediately prior to this panel. The fourth re-arranges terms and the fifth follows by the re-definition of $\tilde{q}_t^{g}$ given by Proposition \ref{prop: stochgform1}, thus providing the result.

To show Corollary \ref{cor: stochgform}, consider that when $\mathbb{A}(g)\subset\mathbb{Z}(g)$ then either $\mathbb{S}(g) = \emptyset$ or else its elements are not necessary to control for confounding (see arguments used in the proof of Lemma \ref{lemma: indgenlemma}). Thus, the conditions of Proposition \ref{prop: stochgform1} hold trivially.
